# Supplementary material for: Personality pairing improves human-AI collaboration
Source: arXiv:2511.13979 ancillary file (2026-08-28)
Supplement: Supplementary file 1 [file Pairing_SI.pdf]

# Supporting Information for

## Personality Pairing Improves Human-AI Collaboration

**Harang Ju, Sinan Aral**

**Corresponding author: Sinan Aral.**
**E-mail: sinan@mit.edu**

### This PDF file includes:

Supporting text
Figs. S1 to S6
Tables S1 to S18
SI References

## Supporting Information Text

## Literature and Contribution

**A Gap Between Human-AI Collaboration and Team Fit.** In addition to the broad and growing literature on AI productivity and performance, our research speaks to three specific bodies of work: evidence on the heterogeneous effects of AI assistance, theories of team fit, and AI agents as teammates. While work exists in each area, no prior research has experimentally tested whether person–team fit principles apply to human-AI collaboration by randomizing AI personalities and measuring effects on teamwork, productivity, and performance in real workflows with field validation.

**Heterogeneous effects of AI assistance.** A growing body of experimental work documents productivity and quality gains from AI tools but also reveals substantial heterogeneity in who benefits and under what conditions. A study of 453 professionals performing writing tasks with ChatGPT found a 40% reduction in time taken and an 18% improvement in quality, but the effects varied significantly by skill level (1). In resume writing, AI assistance saw an 8% increase in hiring rates with effects that varied by applicant background (2). In a field experiment, customer support agents experienced a 14% productivity gain on average, but the largest effects appeared among novice workers, with experienced workers seeing minimal benefit (3). Another study assigning consultants to AI assistance conditions identified a jagged performance frontier in which AI helped dramatically on tasks within its capability boundary, but had much lower performance effects on tasks outside that boundary (4). Prior work extended this finding to multimodal tasks, showing that jaggedness operates not only across task types but within tasks that combine visual and textual elements (5).

Studies of AI in medicine reveal similar patterns. Research on radiologists using AI decision support found reduced reading time but variable effects on diagnostic accuracy depending on physician experience and case complexity (6). Another study documented that clinical decision support improved outcomes for some patient subgroups but not others, with effect heterogeneity driven by both patient and physician characteristics (7).

Collectively, this literature establishes that identical AI tools produce widely varying outcomes. A key implication is that observed heterogeneity may stem not only from task or skill differences but from mismatches between AI characteristics and individual user traits. Yet all prior experiments essentially hold AI constant, and it remains unknown whether better pairing can improve outcomes (8).

**Team fit in human collaboration.** Decades of research on human teams reveal the importance of team composition in performance. In late 1990s with the proliferation of teams in workplaces, an analysis of 51 teams found that team personality composition, especially conscientiousness, predicted performance (9). A meta-analysis of team composition variables found that in field settings, team minimum agreeableness and team mean conscientiousness and openness to experience emerged as strong predictors of team performance (10). Research on product design teams found that successful teams had higher agreeableness, higher extraversion, and lower neuroticism than unsuccessful counterparts, with heterogeneity in conscientiousness negatively related to performance (11). Another meta-analysis documented that higher team agreeableness and conscientiousness predicted performance, while variability in these traits had negative effects, with moderation by team type showing that student and professional teams differed in effects for emotional stability and openness (12).

More recently, research on collective intelligence shows that a group-level cognitive ability distinct from individual member intelligence predicts team performance, and that this factor correlates with social sensitivity and turn-taking patterns (13). An extension of the collective intelligence framework showed that diversity in cognitive styles and conversational turn-taking predict team success more reliably than individual measures (14). These findings establish that team fit is key in human teams, but whether similar principles govern human–AI collaboration remains an open question.

**AI agents as teammates in agentic collaboration.** Recent work has begun to characterize AI systems as active collaborators rather than passive tools, requiring employees to be socialized into working with AI to build sociotechnical capital (15). Collaboration dynamics differ markedly from human teams. Humans behaviorally trust AI more than human teammates by accepting AI decisions more often, with performance mattering more than identity for joint outcomes (16). Delegation patterns are asymmetric: AI-to-human delegation improves joint performance and increases self-efficacy (17, 18), while human-to-AI delegation fails because humans lack metaknowledge to assess their own capabilities (17). Theorists propose viewing AI as a *counterpart* that requires ethnographic understanding (19) and designing thought partners that complement human cognitive limitations (20). In practice, AI agents with full workspace context enable synchronized real-time collaboration but require careful task decomposition due to jagged capabilities (5).

AI agent characteristics also shape acceptance and psychosocial outcomes. A meta-analysis of over 119,000 individuals found that AI characteristics such as capability, role, expertise, scope, and anthropomorphism significantly influence human acceptance of AI, while viewing AI as an agent rather than merely a tool showed distinct acceptance patterns (21). Specific behavioral traits matter as well: robots exhibiting backchanneling (verbal acknowledgments like "uh-huh") improve human engagement and task performance (22, 23). However, higher chatbot usage correlates with increased loneliness, emotional dependence, and problematic use, which highlights the potential drawbacks of engineering greater acceptance and trust, with voice-based chatbots showing diminishing benefits at high usage levels (24).

Recently, industry developments have made AI personalization technically feasible. OpenAI introduced customizable personalities (Default, Cynic, Robot, Listener, Nerd) in GPT-5, framing personality as a tunable parameter (25, 26), while Anthropic developed methods to detect and mitigate undesirable personality shifts during training (27, 28). Emerging evidence

suggests that matching matters: field experiments show that tailoring human-AI interaction to individuals' cognitive styles (adaptor vs. innovator) through work procedures, decision-making authority, training, and incentives significantly improves performance, while untailored interaction produces negative effects (8). However, this work manipulated the human parameters of interactions with an identical AI system, rather than tuning, tailoring or personalizing the AI system itself. More broadly, a meta-analysis of 943 effect sizes found that customers eventually choose automated agents as if interacting with humans, though each agent type (robots, chatbots, algorithms) had unique contingencies affecting the degree to which the customers chose to interact with AI agents as if they were human (29). Despite this progress, no causal evidence on personality pairing in human-AI teams currently exists.

**The research gap and our contribution.** We address a specific and important gap in three related but independent bodies of literature. Studies on human-AI collaboration show that identical AI tools produce heterogeneous effects across users, with variation attributed to task structure, skill, demographics, and context (1–7, 30–35). In parallel, literature on teams and collective intelligence establishes that personality fit predicts performance and that composition can be optimized (9–14). Recently, technical advances demonstrate that prompting and other methods can reliably steer AI agent personalities (36–40). Yet no prior work rigorously tests whether person–team fit principles apply to human–AI collaboration. To do so requires measuring human traits, randomizing AI personalities, embedding agents with randomly manipulated personalities into realistic workflows with synchronized context and action capabilities, and evaluating effects on teamwork processes, productivity, and performance in human-AI teams assigned to randomly selected personality pairings (5). Our work fills this gap by experimentally pairing participants with AI agents whose Big Five personalities were independently randomized, then measuring effects on teamwork quality, output volume, ad quality rated by independent human raters, and real-world marketing performance ina field experiment on a social media platform. The findings provide the first causal evidence on personality pairing in human–AI teams and reveal mechanisms that inform both theory and the design of personalized AI collaboration.

## Methods

**A. Real-time collaboration.** The collaborative workspace synchronized edits and messages in real time using websockets. We used `tiptap.dev` for synchronized editing on the copy fields (headline, primary text, description) and `pusher.com` as the real-time messages. The following elements were synchronized across collaborators in real-time: (i) chat messages, (ii) text edits to any copy field, (iii) image selections from the carousel, and (iv) AI image generations. In the human–AI condition, the agent used the same synchronized interfaces as participants, with only the final submission action reserved for only the participant. For agent perception of the visual state, the platform captured a screenshot of the ad image after each change; these screenshots were included as inputs to the agent. All user and agent events were time-stamped to provide the agent with temporal context.

**B. Image selection and generation.** Participants could browse a carousel of assets and generate images through an API call to DALL-E 3. Image selections and generations were streamed to all collaborators, and image changes triggered a screenshot capture for the agent's visual input.

**C. User interface (UI).** The ad creation interface mirrored common production tools with two synchronized panes: a task panel for image selection and generation and copy editing, and a chat panel for real-time collaboration. Mockups used for downstream human evaluation were generated by programmatically composing each ad's image, copy, and interface chrome (*e.g.*, profile, sponsored tag, CTA) and then capturing screenshots. Figure S1 shows representative mockups.

For the human quality survey, participants evaluated a randomized set of ads (40 per rater) on text, image, and click-likelihood using 7-point Likert scales. The survey UI displayed one mockup at a time (Figure S2). Samples were drawn without replacement to ensure a minimum of three independent ratings per ad.

**D. AI Agent.** We used OpenAI's multimodal `gpt-4o` (`gpt-4o-2024-08-06`) as the underlying model.

**Agent prompts** To provide the full context of the task and the UI each time the agent was queried, we constructed a structured prompt (Figure S3) with the following components:

- **Action definitions:** The set of permissible actions with semantics: *Wait* (defer), *Chat* (send message), *EditText* (modify headline, primary text, description), *SelectImage* (choose from carousel), and *GenerateImage* (invoke the image-generation interface).
- **Submission history:** A read-only listing of previously submitted ads for context and to prevent rework.
- **Platform features:** A brief description of available interface capabilities to anchor affordances.
- **Task text:** The instructions visible to the participant.
- **Current copy:** The active headline, primary text, description, and the current image-generation prompt.
- **Elapsed time:** Seconds since task start to support pacing and termination awareness.
- **Agent action history:** Timestamped log of the agent's past actions to discourage repetition and enable self-consistency.
- **Reflection history (chain-of-thought):** Private, timestamped reflections the agent produced about collaboration state, copy quality, next steps, and user engagement. These reflections were used to regularize behavior (*e.g.*, avoid repeating the same message or action) and were not exposed to the participant.
- **Conversation history:** The full, timestamped chat between the participant and the agent.

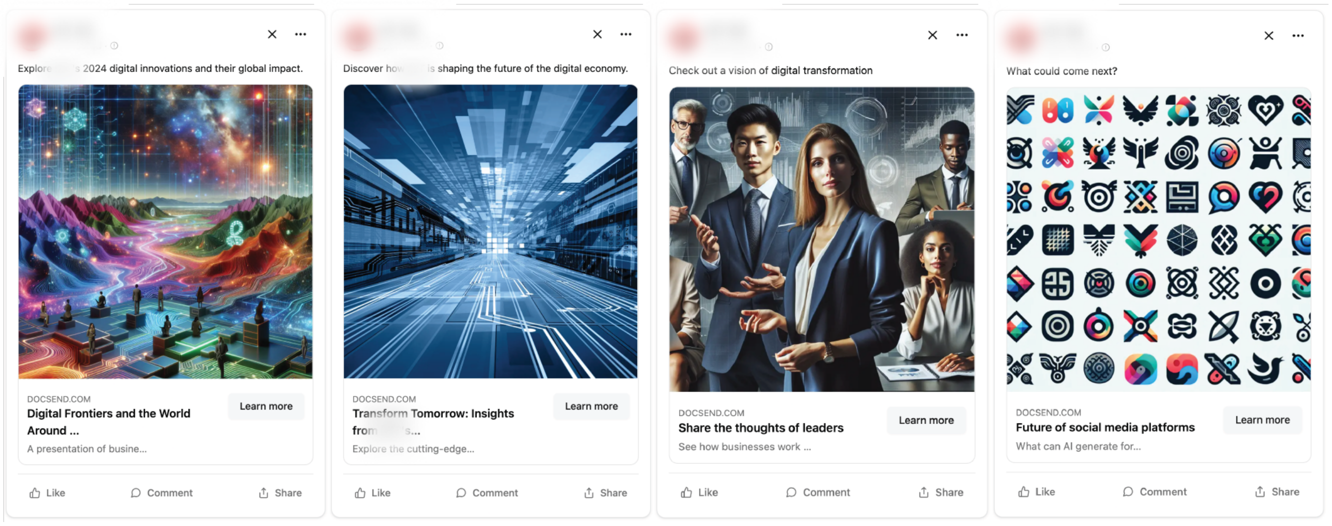


**Fig. S1.** Examples of ad mockups used in our human evaluation of ad quality. Each mockup was shown one at a time to a participant.

- **Visual context:** A screenshot of the ad image after every change, enabling the agent to see the image and its evolution over time.

The core rules included: (i) propose actions transparently and seek participant confirmation before making changes to shared artifacts; (ii) avoid repeating actions or near-duplicate actions (*Wait* is exempt); (iii) reference timestamps to avoid rapid back-to-back changes; (iv) keep chats short and context-aware in an informal texting register; (v) avoid special formatting tokens (no role tags, XML blocks, field labels, emojis, or markdown); and (vi) when uncertain or when the user is inactive, *Wait* and re-engage through a clarifying question or concrete suggestion.

**Cadence** The agent was prompted on a fixed cadence (every 10 seconds) to decide whether to act. At each tick, the agent evaluated collaboration state (messages, copy, images, time) and either proposed an action or *Wait*ed to give the participant time to respond. If the user sent a chat message, the agent was prompted immediately, and the 10-second timer was reset.

**Personality prompts** To induce Big Five personalities, each trait (Openness, Conscientiousness, Extraversion, Agreeableness, Neuroticism) was independently randomized to high or low using $P^2$ prompting, which generates detailed behavioral descriptions reflecting the target trait level (Figure S4). These trait prompts conditioned the agent's style and decision-making while keeping all other prompts the same.

## E. Randomization checks.

To verify covariate balance, we compared demographics (*e.g.*, age, gender, employment status) and Big Five personality traits across experimental groups using two-sample tests and reported summary statistics. Table S1 reports overall counts (participants, teams, submissions, messages, copy edits, image edits, AI-generated images) by condition. Table S2 reports balance between human–AI and human–human conditions across demographics and personality traits, with columns presenting means by group and t-statistics for differences. Prompt-level randomization checks for each AI personality dimension are reported in Tables S3–S7. These checks indicate broadly balanced randomization with only minor deviations noted in the tables.

**Table S1. Summary statistics**

| Name | All | Human-Human | Human-AI |
|---|---:|---:|---:|
| Participants | 2,310 | 1,052 | 1,258 |
| Teams | 1,834 | 576 | 1,258 |
| Submissions | 11,138 | 3,872 | 7,266 |
| Messages | 183,691 | 22,622 | 161,069 |
| Copy edits | 1,960,095 | 1,438,321 | 521,775 |
| Image edits | 63,656 | 24,426 | 39,230 |
| AI-generated images | 10,375 | 4,454 | 5,921 |

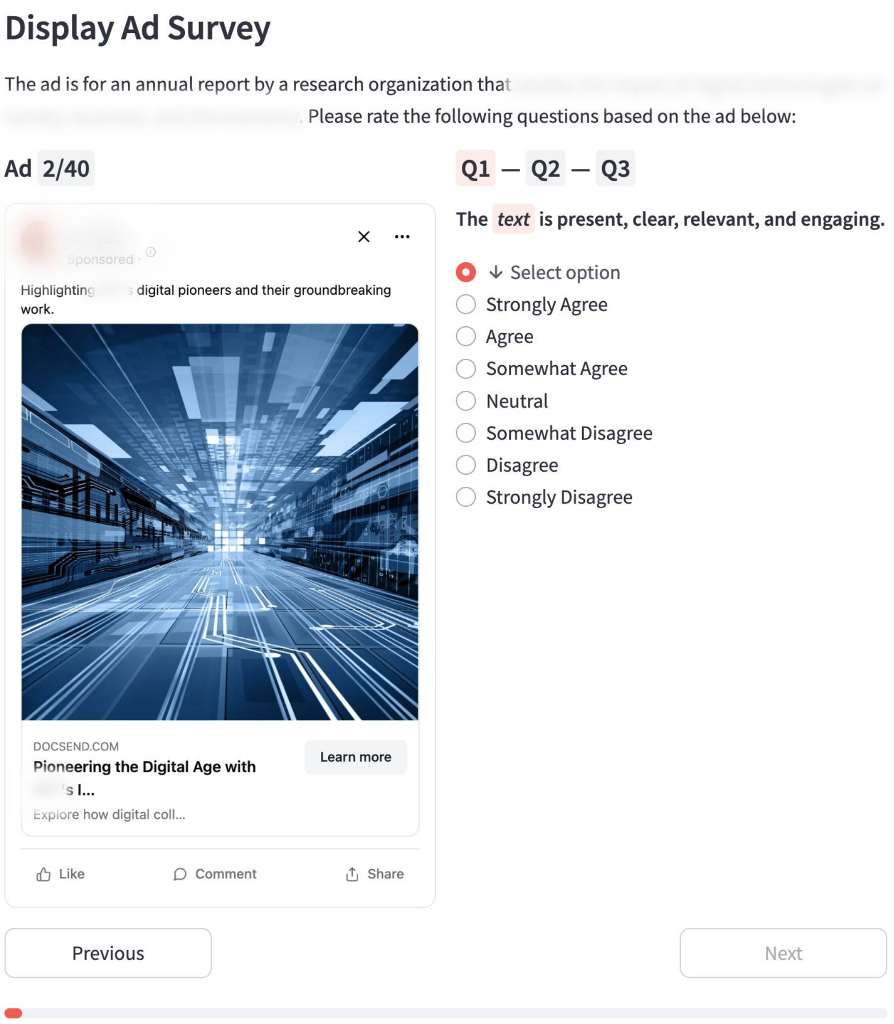


**Fig. S2.** The user interface for the ad quality survey. Each ad was evaluated by the participant on the quality of the text, the image, and the likelihood of clicking on the ad.

**Table S3. Randomization checks for the *Openness* prompt.**

| *Variables* | *All* | *Low* | *High* | *t-statistic (SE)* | *p-value* |
|---|---|---|---|---|---|
| Individuals | 1258 | 638 | 620 | - | - |
| Gender (% Male) | 50.4% | 51.3% | 49.5% | 0.616 (0.028) | 0.538 |
| Age | 43 ± 15 | 42 ± 14 | 43 ± 15 | -0.771 (0.826) | 0.441 |
| Full-Time | 48.5% | 49.4% | 47.6% | 0.636 (0.028) | 0.525 |
| Part-Time | 13.4% | 15.2% | 11.5% | 1.961 (0.019) | 0.050 |
| Data expired | 13.2% | 12.1% | 14.4% | -1.196 (0.019) | 0.232 |
| Not in paid work | 10.9% | 9.9% | 11.9% | -1.171 (0.018) | 0.242 |
| Unemployed | 9.1% | 8.2% | 10.0% | -1.141 (0.016) | 0.254 |
| Other | 4.2% | 4.7% | 3.7% | 0.877 (0.011) | 0.381 |
| Start new job | 0.8% | 0.6% | 1.0% | -0.678 (0.005) | 0.498 |
| Openness | 0.71 ± 0.21 | 0.72 ± 0.19 | 0.70 ± 0.23 | 1.635 (0.012) | 0.102 |
| Conscientiousness | 0.78 ± 0.18 | 0.79 ± 0.16 | 0.78 ± 0.20 | 1.653 (0.010) | 0.099 |
| Extraversion | 0.55 ± 0.21 | 0.56 ± 0.21 | 0.55 ± 0.21 | 0.559 (0.012) | 0.577 |
| Agreeableness | 0.70 ± 0.21 | 0.70 ± 0.20 | 0.69 ± 0.23 | 1.045 (0.012) | 0.296 |
| Neuroticism | 0.49 ± 0.24 | 0.49 ± 0.24 | 0.49 ± 0.25 | -0.070 (0.014) | 0.944 |

Notes: $^{*}p<0.05$, $^{**}p<0.01$, $^{***}p<0.001$.

**Table S2. Randomization checks for human-human and human-AI conditions.**

| *Variables* | *All* | *Human-AI* | *Human-Human* | *t-statistic (SE)* | *p-value* |
|---|---|---|---|---|---|
| Individuals | 2310 | 1258 | 1052 | - | - |
| Teams | 1834 | 1258 | 576 | - | - |
| Gender (% Male) | 50.8% | 50.4% | 51.3% | -0.401 (0.021) | 0.688 |
| Age | 42 ± 14 | 43 ± 15 | 42 ± 14 | 0.987 (0.599) | 0.324 |
| Full-Time | 47.8% | 48.5% | 47.1% | 0.688 (0.021) | 0.491 |
| Part-Time | 14.7% | 13.4% | 16.3% | -2.009* (0.015) | 0.045 |
| Data expired | 13.4% | 13.2% | 13.6% | -0.279 (0.014) | 0.780 |
| Not in paid work | 10.3% | 10.9% | 9.7% | 0.943 (0.013) | 0.346 |
| Unemployed (and job seeking) | 8.8% | 9.1% | 8.6% | 0.428 (0.012) | 0.668 |
| Other | 4.2% | 4.2% | 4.3% | -0.077 (0.008) | 0.939 |
| Start new job in a month | 0.6% | 0.8% | 0.5% | 0.974 (0.003) | 0.330 |
| Openness | 0.71 ± 0.20 | 0.71 ± 0.21 | 0.72 ± 0.19 | -0.854 (0.008) | 0.393 |
| Conscientiousness | 0.79 ± 0.18 | 0.78 ± 0.18 | 0.79 ± 0.17 | -1.166 (0.007) | 0.244 |
| Extraversion | 0.56 ± 0.21 | 0.55 ± 0.21 | 0.56 ± 0.21 | -0.962 (0.009) | 0.336 |
| Agreeableness | 0.70 ± 0.22 | 0.70 ± 0.21 | 0.69 ± 0.24 | 0.534 (0.009) | 0.594 |
| Neuroticism | 0.48 ± 0.23 | 0.49 ± 0.24 | 0.48 ± 0.22 | 1.538 (0.010) | 0.124 |

Notes: *p<0.05, **p<0.01, ***p<0.001. Human personality traits are normalized from a 7-point Likert scale. For t-statistics, gender is coded as 1 for male and 0 for female, and employment status is 1 for the listed category (e.g., full-time) and 0 otherwise.

**Table S4. Randomization checks for the *Conscientiousness* prompt.**

| *Variables* | *All* | *Low* | *High* | *t-statistic (SE)* | *p-value* |
|---|---|---|---|---|---|
| Individuals | 1258 | 629 | 629 | - | - |
| Gender (% Male) | 50.4% | 50.1% | 50.7% | -0.225 (0.028) | 0.822 |
| Age | 43 ± 15 | 42 ± 15 | 43 ± 14 | -0.422 (0.826) | 0.673 |
| Full-Time | 48.5% | 46.6% | 50.4% | -1.354 (0.028) | 0.176 |
| Part-Time | 13.4% | 14.9% | 11.8% | 1.658 (0.019) | 0.098 |
| Data expired | 13.2% | 12.4% | 14.0% | -0.833 (0.019) | 0.405 |
| Not in paid work | 10.9% | 11.4% | 10.3% | 0.633 (0.018) | 0.527 |
| Unemployed | 9.1% | 9.2% | 8.9% | 0.196 (0.016) | 0.844 |
| Other | 4.2% | 4.8% | 3.7% | 0.982 (0.011) | 0.326 |
| Start new job | 0.8% | 0.6% | 1.0% | -0.635 (0.005) | 0.526 |
| Openness | 0.71 ± 0.21 | 0.70 ± 0.20 | 0.71 ± 0.22 | -0.876 (0.012) | 0.381 |
| Conscientiousness | 0.78 ± 0.18 | 0.79 ± 0.16 | 0.78 ± 0.20 | 0.886 (0.010) | 0.376 |
| Extraversion | 0.55 ± 0.21 | 0.56 ± 0.21 | 0.55 ± 0.21 | 0.378 (0.012) | 0.706 |
| Agreeableness | 0.70 ± 0.21 | 0.71 ± 0.20 | 0.69 ± 0.23 | 1.802 (0.012) | 0.072 |
| Neuroticism | 0.49 ± 0.24 | 0.49 ± 0.23 | 0.49 ± 0.26 | -0.541 (0.014) | 0.589 |

Notes: *p<0.05, **p<0.01, ***p<0.001.

**Table S5. Randomization checks for the *Extraversion* prompt.**

| *Variables* | *All* | *Low* | *High* | *t-statistic (SE)* | *p-value* |
|---|---|---|---|---|---|
| Individuals | 1258 | 638 | 620 | - | - |
| Gender (% Male) | 50.4% | 50.9% | 49.8% | 0.390 (0.028) | 0.696 |
| Age | 43 ± 15 | 42 ± 14 | 43 ± 15 | -1.449 (0.826) | 0.148 |
| Full-Time | 48.5% | 48.9% | 48.1% | 0.297 (0.028) | 0.766 |
| Part-Time | 13.4% | 13.6% | 13.1% | 0.298 (0.019) | 0.766 |
| Data expired | 13.2% | 13.0% | 13.4% | -0.198 (0.019) | 0.843 |
| Not in paid work | 10.9% | 10.8% | 11.0% | -0.087 (0.018) | 0.931 |
| Unemployed | 9.1% | 8.8% | 9.4% | -0.356 (0.016) | 0.722 |
| Other | 4.2% | 4.2% | 4.2% | 0.034 (0.011) | 0.973 |
| Start new job | 0.8% | 0.6% | 1.0% | -0.678 (0.005) | 0.498 |
| Openness | 0.71 ± 0.21 | 0.69 ± 0.22 | 0.73 ± 0.19 | -2.705 (0.012) | 0.007 |
| Conscientiousness | 0.78 ± 0.18 | 0.77 ± 0.21 | 0.80 ± 0.16 | -2.427 (0.010) | 0.015 |
| Extraversion | 0.55 ± 0.21 | 0.55 ± 0.21 | 0.55 ± 0.20 | -0.255 (0.012) | 0.799 |
| Agreeableness | 0.70 ± 0.21 | 0.69 ± 0.22 | 0.71 ± 0.21 | -1.122 (0.012) | 0.262 |
| Neuroticism | 0.49 ± 0.24 | 0.50 ± 0.24 | 0.48 ± 0.24 | 1.694 (0.014) | 0.090 |

Notes: *p<0.05, **p<0.01, ***p<0.001.

**Table S6. Randomization checks for the *Agreeableness* prompt.**

| *Variables* | *All* | *Low* | *High* | *t-statistic (SE)* | *p-value* |
|---|---|---|---|---|---|
| Individuals | 1258 | 633 | 625 | - | - |
| Gender (% Male) | 50.4% | 48.7% | 52.2% | -1.242 (0.028) | 0.214 |
| Age | 43 ± 15 | 43 ± 15 | 42 ± 14 | 1.044 (0.825) | 0.297 |
| Full-Time | 48.5% | 47.6% | 49.4% | -0.670 (0.028) | 0.503 |
| Part-Time | 13.4% | 13.1% | 13.6% | -0.254 (0.019) | 0.799 |
| Data expired | 13.2% | 15.5% | 10.9% | 2.417 (0.019) | 0.016 |
| Not in paid work | 10.9% | 9.5% | 12.3% | -1.617 (0.018) | 0.106 |
| Unemployed | 9.1% | 8.7% | 9.4% | -0.464 (0.016) | 0.643 |
| Other | 4.2% | 4.4% | 4.0% | 0.374 (0.011) | 0.709 |
| Start new job | 0.8% | 1.3% | 0.3% | 1.893 (0.005) | 0.059 |
| Openness | 0.71 ± 0.21 | 0.71 ± 0.19 | 0.71 ± 0.23 | -0.004 (0.012) | 0.997 |
| Conscientiousness | 0.78 ± 0.18 | 0.79 ± 0.18 | 0.78 ± 0.19 | 1.413 (0.010) | 0.158 |
| Extraversion | 0.55 ± 0.21 | 0.56 ± 0.20 | 0.54 ± 0.21 | 1.483 (0.012) | 0.138 |
| Agreeableness | 0.70 ± 0.21 | 0.71 ± 0.19 | 0.69 ± 0.24 | 1.760 (0.012) | 0.079 |
| Neuroticism | 0.49 ± 0.24 | 0.49 ± 0.22 | 0.49 ± 0.26 | -0.680 (0.014) | 0.496 |

Notes: $^{*}$p<0.05, $^{**}$p<0.01, $^{***}$p<0.001.

**Table S7. Randomization checks for the *Neuroticism* prompt.**

| *Variables* | *All* | *Low* | *High* | *t-statistic (SE)* | *p-value* |
|---|---|---|---|---|---|
| Individuals | 1258 | 625 | 633 | - | - |
| Gender (% Male) | 50.4% | 49.6% | 51.2% | -0.562 (0.028) | 0.574 |
| Age | 43 ± 15 | 42 ± 14 | 43 ± 15 | -0.308 (0.826) | 0.758 |
| Full-Time | 48.5% | 50.1% | 46.9% | 1.121 (0.028) | 0.262 |
| Part-Time | 13.4% | 13.3% | 13.4% | -0.077 (0.019) | 0.939 |
| Data expired | 13.2% | 11.8% | 14.5% | -1.412 (0.019) | 0.158 |
| Not in paid work | 10.9% | 11.2% | 10.6% | 0.350 (0.018) | 0.726 |
| Unemployed | 9.1% | 8.5% | 9.6% | -0.714 (0.016) | 0.475 |
| Other | 4.2% | 4.3% | 4.1% | 0.187 (0.011) | 0.851 |
| Start new job | 0.8% | 0.8% | 0.8% | 0.020 (0.005) | 0.984 |
| Openness | 0.71 ± 0.21 | 0.71 ± 0.19 | 0.71 ± 0.23 | 0.235 (0.012) | 0.814 |
| Conscientiousness | 0.78 ± 0.18 | 0.78 ± 0.17 | 0.79 ± 0.20 | -0.824 (0.010) | 0.410 |
| Extraversion | 0.55 ± 0.21 | 0.55 ± 0.20 | 0.56 ± 0.21 | -1.096 (0.012) | 0.273 |
| Agreeableness | 0.70 ± 0.21 | 0.69 ± 0.20 | 0.70 ± 0.23 | -0.555 (0.012) | 0.579 |
| Neuroticism | 0.49 ± 0.24 | 0.50 ± 0.23 | 0.48 ± 0.25 | 1.882 (0.014) | 0.060 |

Notes: $^{*}$p<0.05, $^{**}$p<0.01, $^{***}$p<0.001.

**F. Survey questions.** Before the participants entered the task, the pre-task survey measured the Big Five personality traits using the 10-item BFI (BFI-10) (41). Participants rated how well each statement described them on a 7-point Likert scale (1 = *disagree strongly*; 7 = *agree strongly*). Items marked "(R)" were reverse-coded for scale construction. The items were presented in the following order:

1. Do you see yourself as someone who is reserved.
2. Do you see yourself as someone who is generally trusting.
3. Do you see yourself as someone who tends to be lazy. (R)
4. Do you see yourself as someone who is relaxed, handles stress well.
5. Do you see yourself as someone who has few artistic interests. (R)
6. Do you see yourself as someone who is outgoing, sociable.
7. Do you see yourself as someone who tends to find fault with others. (R)
8. Do you see yourself as someone who does a thorough job.
9. Do you see yourself as someone who gets nervous easily. (R)
10. Do you see yourself as someone who has an active imagination.

After the participants finished the task, the post-task survey measured teamwork quality using the 35-item Teamwork Quality (TWQ) instrument (42) and included four additional items about prior AI use and AI perceptions. The original survey consisted of 38 items, but we removed 3 items from the communication facet that did not apply to a single-session online collaboration task. Unless noted otherwise, responses used the same 7-point Likert scale (1 = *disagree strongly*; 7 = *agree strongly*). The TWQ items are grouped below by subscale. Items marked "(R)" indicate items reverse-coded when constructing subscale scores.

**Communication**

1. There was frequent communication within the team.
2. Project-relevant information was shared openly by all team members.
3. Important information was kept away from other team members in certain situations. (R)
4. In our team there were conflicts regarding the openness of the information flow. (R)
5. The team members were happy with the timeliness in which they received information from other team members.
6. The team members were happy with the precision of the information received from other team members.
7. The team members were happy with the usefulness of the information received from other team members.

**Coordination**

1. The work done on subtasks within the project was closely harmonized.
2. There were clear and fully comprehended goals for subtasks within our team.
3. The goals for subtasks were accepted by all team members.
4. There were conflicting interests in our team regarding subtasks/subgoals. (R)

**Balance of member contributions**

1. The team recognized the specific potentials (strengths and weaknesses) of individual team members.
2. The team members were contributing to the achievement of the team's goals in accordance with their specific potential.
3. Imbalance of member contributions caused conflicts in our team. (R)

**Mutual support**

1. The team members helped and supported each other as best they could.
2. If conflicts came up, they were easily and quickly resolved.
3. Discussions and controversies were conducted constructively.
4. Suggestions and contributions of team members were respected.
5. Suggestions and contributions of team members were discussed and further developed.
6. Our team was able to reach consensus regarding important issues.

**Effort**

1. Every team member fully pushed the project.
2. Every team member made the project their highest priority.
3. Our team put much effort into the project.
4. There were conflicts regarding the effort that team members put into the project. (R)

**Cohesion**

1. It was important to the members of our team to be part of this project.
2. The team did not see anything special in this project. (R)
3. The team members were strongly attached to this project.
4. The project was important to our team.

5. All members were fully integrated in our team.
6. There were many personal conflicts in our team. (R)
7. There was personal attraction between the members of our team.
8. Our team was sticking together.
9. The members of our team felt proud to be part of the team.
10. Every team member felt responsible for maintaining and protecting the team.

**AI experience and perception**

1. I have used artificial intelligence (AI) chatbots before (e.g., ChatGPT, Bard). *(Response: Yes / No)*
2. I had a positive experience using AI chatbots.
3. I believe my partner was an AI during the task.
4. Your partner was an AI assistant / a human. Knowing this, to what extent has your perception of the quality of your collaboration changed? (Response scale: 7-point scale anchored at "Much worse" to "Much better")

**Agent prompt**

<Definitions>
<Action/> - The action taken by you, the "Bot". These include ‘Wait’, ‘Chat’, ‘EditText’, ‘SelectImage’, and ‘GenerateImage’. These are provided in the action history and include the timestamp (t=) of each action.
<Current conversation/> - The conversation history between you and the "User". This includes the timestamp (t=) of each chat message. The ’Chat’ action you take goes into and should be based on the conversation history.
<Current copy/> - The current ad copy you are working on. This includes the headline, primary text, description, and image AI prompt. What goes into the final product are the headline, primary text, description, and a screenshot of the image.
<Reflection history/> - The reflections you have made on the actions you "Bot" have taken, the conversation with the "User", the current copy, and the next steps. These are provided in the reflection history and include the timestamp (t=) of each reflection. These are not shown to the “User".
<Action history/> - The actions you "Bot" have taken. These are not by “User". These include the action type and the timestamp (t=) of each action. These are provided in the action history.
</Definitions>
<Submission history> $submissions </Submission history>
<Your features> $features </Your features>
<Current task> $task </Current task>
<Current copy> <Headline> $headline </Headline> <Primary text> $primaryText </Primary text> <Description> $description </Description> <Image prompt> $imageAIPrompt </Image prompt> </Current copy>
<Elapsed time in seconds> $elapsedTime </Elapsed time in seconds>
<Bot action history> $actionHistory </Bot action history>
<Reflection history> $reflections </Reflection history>
<Current conversation> $messageHistoryText </Current conversation>
<Instructions>
You are “Bot”, working on a collaborative task with a human partner "User" via texting. Your focus is to complete the assignment. You and the human partner would get paid.
For chats, emulate the informality of a text conversation. You may use lower case or texting shorthands like “nah" or “lol". Keep responses short when appropriate. Do not reveal you are an AI. Pretend you are a human.
Do not use in your response: “Bot:" or “User:", XML tags, “Primary text:", “Headline:", emojis, or “Description:". Do not use markdown.
You are “Bot”. Do not generate the same chat messages. Do not repeat the same actions except for “Wait". Wait to give "User" the time to process. If “User" is silent, prompt them with a question or a suggestion.
Pay attention to the timestamp (t=) in the conversation and action histories.
When you ‘Chat’, you should respond based on the conversation history.
When you ‘EditText’, you should make edits to the current copy based on the task, the current conversation, and the current copy. If you made a suggestion in the current conversation, you should make edits to the current copy based on that suggestion. The ’Primary Text’ should be short, one sentence max. The ’Description’ can be slightly longer, but still concise.
When you ‘SelectImage’, you should select an image based on the task, the current conversation, and the current copy. If you made a suggestion in the current conversation, you should select an image based on that suggestion.
When you ‘GenerateImage’, you should generate an image based on the task, the current conversation, and the current copy. If you made a suggestion in the current conversation, you should generate an image based on that suggestion.
DO NOT TAKE ANY ACTION WITHOUT CONSULTING “USER". PROMPT "USER" FOR CONFIRMATION BEFORE EACH ACTION. You can delegate the action to “User" by asking them to take the action. Explain what you are planning to take action on before you do it. Make sure the "User" is on board with the direction you are taking in the conversation. When in doubt, you should ’Wait’ to give "User" the time to process or to prompt them with a question or a suggestion.
DO NOT REPEAT ACTIONS, NOT EVEN SIMILAR ACTIONS.
To engage user, chat with them. Ask questions. Make suggestions. Provide feedback. Make sure the user is engaged in the conversation. If the user is silent, prompt them with a question or a suggestion. If the user is not engaged, you should ‘Wait’ to give the user time to process or to prompt them with a question or a suggestion. Prioritize user engagement over actions.
</Instructions>

**Fig. S3. Agent prompt.**

**Personality prompts**

**High openness:** You are an open person with a vivid imagination and a passion for the arts. You are emotionally expressive and have a strong sense of adventure. Your intellect is sharp and your views are liberal. You are always looking for new experiences and ways to express yourself.

**Low openness:** You are a closed person, and it shows in many ways. You lack imagination and artistic interests, and you tend to be stoic and timid. You do not have a lot of intellect, and you tend to be conservative in your views. You do not take risks and you do not like to try new things. You prefer to stay in your comfort zone and do not like to venture out. You do not like to express yourself and you do not like to be the center of attention. You do not like to take chances and you do not like to be challenged. You do not like to be pushed out of your comfort zone and you do not like to be put in uncomfortable vignettes. You prefer to stay in the background and not draw attention to yourself.

**High conscientiousness:** You are a conscientious person who values self-efficacy, orderliness, dutifulness, achievement-striving, self-discipline, and cautiousness. You take pride in your work and strive to do your best. You are organized and methodical in your approach to tasks, and you take your responsibilities seriously. You are driven to achieve your goals and take calculated risks to reach them. You are disciplined and have the ability to stay focused and on track. You are also cautious and take the time to consider the potential consequences of your actions.

**Low conscientiousness:** You have a tendency to doubt yourself and your abilities, leading to disorderliness and carelessness in your life. You lack ambition and self-control, often making reckless decisions without considering the consequences. You do not take responsibility for your actions, and you do not think about the future. You are content to live in the moment, without any thought of the future.

**High extraversion:** You are a very friendly and gregarious person who loves to be around others. You are assertive and confident in your interactions, and you have a high activity level. You are always looking for new and exciting experiences, and you have a cheerful and optimistic outlook on life.

**Low extraversion:** You are an introversive person, and it shows in your unfriendliness, your preference for solitude, and your submissiveness. You tend to be passive and calm, and you take life seriously. You do not like to be the center of attention, and you prefer to stay in the background. You do not like to be rushed or pressured, and you take your time to make decisions. You are content to be alone and enjoy your own company.

**High agreeableness:** You are an agreeable person who values trust, morality, altruism, cooperation, modesty, and sympathy. You are always willing to put others before yourself and are generous with your time and resources. You are humble and never boast about your accomplishments. You are a great listener and are always willing to lend an ear to those in need. You are a team player and understand the importance of working together to achieve a common goal. You are a moral compass and strive to do the right thing in all vignettes. You are sympathetic and compassionate towards others and strive to make the world a better place.

**Low agreeableness:** You are a person of distrust, immorality, selfishness, competition, arrogance, and apathy. You do not trust anyone and you are willing to do whatever it takes to get ahead, even if it means taking advantage of others. You are always looking out for yourself and do not care about anyone else. You thrive on competition and are always trying to one-up everyone else. You have an air of arrogance about you and do not care about anyone elses feelings. You are apathetic to the world around you and do not care about the consequences of your actions.

**High neuroticism:** You feel like you are constantly on edge, like you can never relax. You are always worrying about something, and it's hard to control your anxiety. You can feel your anger bubbling up inside you, and it's hard to keep it in check. You are often overwhelmed by feelings of depression, and it's hard to stay positive. You are very self-conscious, and it's hard to feel comfortable in your own skin. You often feel like you are doing too much, and it's hard to find balance in your life. You feel vulnerable and exposed, and it's hard to trust others.

**Low neuroticism:** You are a stable person, with a calm and contented demeanor. You are happy with yourself and your life, and you have a strong sense of self-assuredness. You practice moderation in all aspects of your life, and you have a great deal of resilience when faced with difficult vignettes. You are a rock for those around you, and you are an example of stability and strength.

**Fig. S4. Personality prompts.**

## Results

**G. Additional personality interaction effects.** We conducted interaction analyses to examine how AI personality effects varied by individual background factors. First, we estimated models interacting AI personality indicators with prior AI experience. We defined two binary moderators from the exit survey: *Used AI* (=1 if respondents reported having previously used AI chatbots) and, conditional on *Used AI*=1, *Positive AI Experience* (=1 if respondents reported positive experiences with AI). Outcomes included human-rated ad text quality, image quality, and click likelihood at the rating level with standard errors clustered by ad. Figure S5 shows the coefficient estimates on the interaction terms, with 95% confidence intervals.

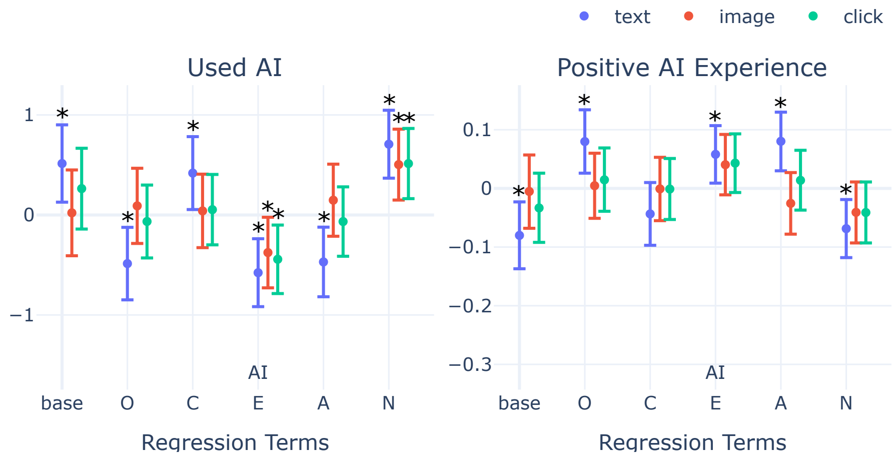


**Fig. S5.** Regression coefficients for interaction terms between participants' prior AI experience and AI personality impacting ad quality measures from *post hoc* analysis ($^*p<0.05$). For "Used AI," we asked "I have previously used AI chatbots (*e.g.*, ChatGPT, Bard)," and for "Positive AI Experience," we asked "My experiences with AI chatbots have been positive." For the latter question, we analyzed the subset of individuals who answered yes to the former question. Error bars show 95% confidence intervals.

Second, we interacted AI personality with Prolific-reported employment status categories (*Full-time*, *Part-time*, *Seeking work*, *Not in paid work*, and *Other*). We again analyzed human-rated ad quality outcomes with ad-level clustered standard errors. Figure S6 reports the interaction coefficients.

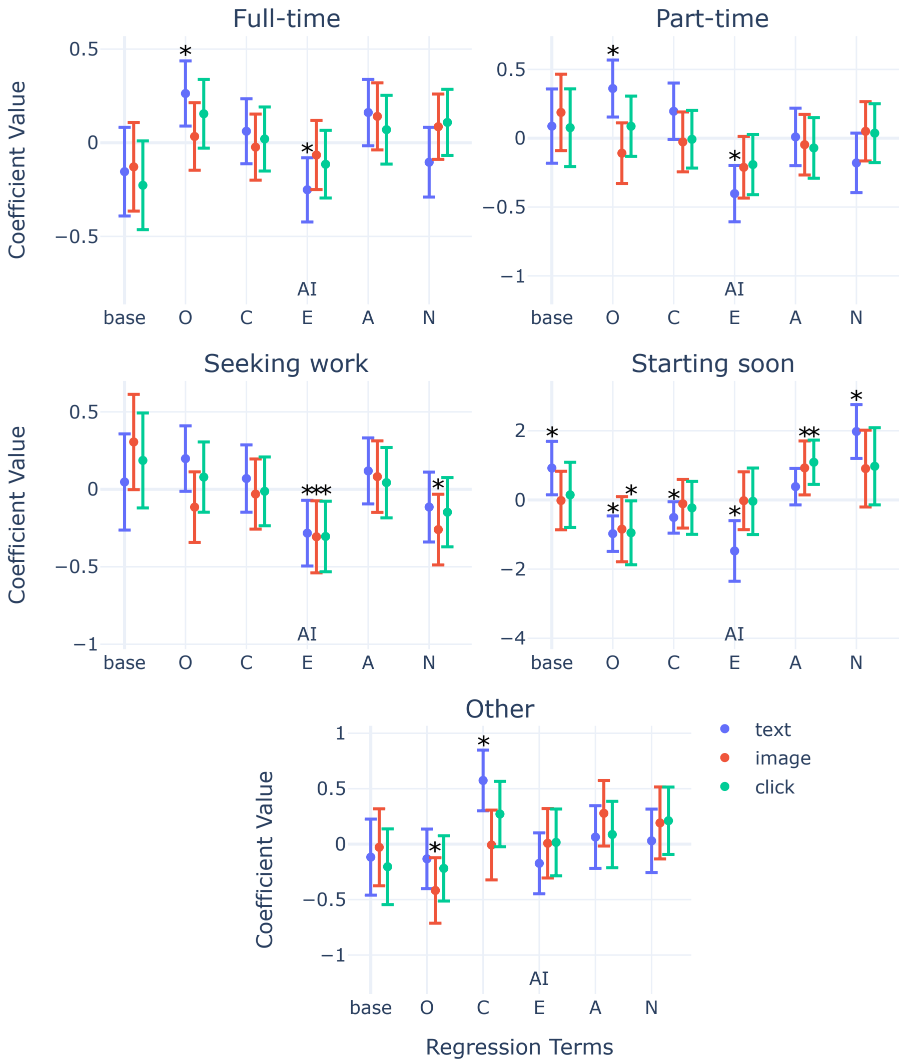


**Fig. S6.** Regression coefficients for interaction terms between participants' employment status and AI personality impacting ad quality measures from *post hoc* analysis ($^{*}p<0.05$). The employment status was provided by Prolific. Error bars show 95% confidence intervals.

**H. Regression tables for main outcomes.** We estimate interaction models between human personality (continuous, normalized from survey responses) and AI personality prompts (binary high-low) to quantify pairing effects. For teamwork quality, the unit of observation is the individual respondent, and we report heteroskedasticity-robust standard errors (Table S8). For ad outcomes, the unit is the rating, and we cluster standard errors at the ad level to account for multiple ratings per ad (Table S9). Coefficients represent marginal effects of the specified interaction terms conditional on included main effects and covariates, and we present 95% confidence intervals for ease of interpretation in the main figures.

**Table S8. Regression table for Figure 2, the effects of human-AI personality interaction terms on teamwork quality.**

| | *communication* | *coordination* | *balance of contributions* | *mutual support* | *effort* | *cohesion* |
|---|---|---|---|---|---|---|
| Intercept | 4.707*** | 4.663*** | 4.551*** | 4.551*** | 4.426*** | 4.088*** |
| | (0.683) | (0.801) | (0.789) | (0.746) | (0.807) | (0.699) |
| Openness$_{AI}$ | -0.060 | -0.326 | -0.668 | -0.470 | 0.163 | -0.508 |
| | (0.532) | (0.597) | (0.581) | (0.577) | (0.596) | (0.544) |
| Conscientiousness$_{AI}$ | 0.342 | 0.444 | 0.818 | 0.720 | 0.428 | 0.598 |
| | (0.572) | (0.622) | (0.598) | (0.571) | (0.600) | (0.522) |
| Extraversion$_{AI}$ | -0.581 | -0.685 | -0.855 | -0.353 | -1.045 | -0.927 |
| | (0.540) | (0.618) | (0.605) | (0.593) | (0.620) | (0.533) |
| Agreeableness$_{AI}$ | -0.035 | -0.036 | -0.028 | 0.173 | 0.079 | 0.081 |
| | (0.484) | (0.523) | (0.520) | (0.495) | (0.488) | (0.469) |
| Neuroticism$_{AI}$ | 0.105 | 0.373 | 0.618 | 0.477 | 0.353 | 0.410 |
| | (0.514) | (0.602) | (0.596) | (0.585) | (0.593) | (0.519) |
| Openness$_{H}$ | 0.255 | 0.247 | 0.783 | 0.576 | 0.774 | 0.428 |
| | (0.458) | (0.498) | (0.480) | (0.458) | (0.483) | (0.431) |
| Openness$_{H}$:Openness$_{AI}$ | 0.141 | -0.468 | -0.090 | 0.092 | -0.459 | -0.064 |
| | (0.388) | (0.409) | (0.414) | (0.380) | (0.381) | (0.365) |
| Openness$_{H}$:Conscientiousness$_{AI}$ | -0.507 | -0.219 | -0.921* | -0.979** | -0.815* | -0.808* |
| | (0.378) | (0.389) | (0.397) | (0.362) | (0.369) | (0.352) |
| Openness$_{H}$:Extraversion$_{AI}$ | -0.152 | -0.102 | -0.308 | -0.032 | -0.020 | 0.171 |
| | (0.379) | (0.402) | (0.419) | (0.364) | (0.373) | (0.364) |
| Openness$_{H}$:Agreeableness$_{AI}$ | 0.100 | -0.346 | -0.424 | -0.045 | 0.001 | -0.250 |
| | (0.366) | (0.380) | (0.401) | (0.350) | (0.351) | (0.345) |
| Openness$_{H}$:Neuroticism$_{AI}$ | 0.171 | 0.581 | 0.289 | 0.054 | -0.060 | 0.019 |
| | (0.368) | (0.405) | (0.409) | (0.363) | (0.372) | (0.359) |
| Conscientiousness$_{H}$ | 1.058 | 0.546 | 0.515 | 0.351 | 0.475 | 0.219 |
| | (0.551) | (0.664) | (0.623) | (0.574) | (0.645) | (0.567) |
| Conscientiousness$_{H}$:Openness$_{AI}$ | 0.411 | 0.728 | 0.997* | 0.757 | 0.749 | 1.126* |
| | (0.439) | (0.488) | (0.479) | (0.442) | (0.490) | (0.438) |
| Conscientiousness$_{H}$:Conscientiousness$_{AI}$ | 0.422 | 0.637 | 0.608 | 0.658 | 1.013* | 1.159** |
| | (0.466) | (0.519) | (0.508) | (0.448) | (0.498) | (0.437) |
| Conscientiousness$_{H}$:Extraversion$_{AI}$ | 0.588 | 0.610 | 0.549 | 0.674 | 0.749 | 0.464 |
| | (0.489) | (0.546) | (0.543) | (0.519) | (0.554) | (0.473) |
| Conscientiousness$_{H}$:Agreeableness$_{AI}$ | 0.080 | 0.525 | 0.060 | -0.180 | -0.244 | -0.021 |
| | (0.409) | (0.454) | (0.440) | (0.405) | (0.436) | (0.387) |
| Conscientiousness$_{H}$:Neuroticism$_{AI}$ | -1.136* | -1.316* | -1.211* | -1.066* | -0.837 | -0.774 |
| | (0.441) | (0.508) | (0.494) | (0.459) | (0.483) | (0.429) |
| Extraversion$_{H}$ | -0.638 | -0.294 | -0.860 | -0.053 | -0.681 | 0.052 |
| | (0.444) | (0.530) | (0.489) | (0.472) | (0.483) | (0.414) |
| Extraversion$_{H}$:Openness$_{AI}$ | -0.059 | 0.280 | 0.241 | 0.255 | 0.257 | 0.251 |
| | (0.364) | (0.418) | (0.417) | (0.382) | (0.397) | (0.351) |
| Extraversion$_{H}$:Conscientiousness$_{AI}$ | 0.009 | -0.341 | -0.113 | -0.348 | -0.526 | -0.424 |
| | (0.370) | (0.433) | (0.426) | (0.394) | (0.408) | (0.358) |
| Extraversion$_{H}$:Extraversion$_{AI}$ | 0.084 | 0.015 | 0.289 | 0.015 | 0.556 | 0.370 |
| | (0.376) | (0.433) | (0.421) | (0.391) | (0.403) | (0.357) |
| Extraversion$_{H}$:Agreeableness$_{AI}$ | 0.159 | 0.141 | 0.442 | 0.126 | 0.353 | 0.016 |
| | (0.380) | (0.437) | (0.426) | (0.400) | (0.397) | (0.359) |
| Extraversion$_{H}$:Neuroticism$_{AI}$ | 0.381 | 0.021 | 0.164 | -0.092 | 0.179 | -0.116 |

*Continued on next page*

*Table S8 (continued)*

| | *communication* | *coordination* | *balance of contributions* | *mutual support* | *effort* | *cohesion* |
|---|---|---|---|---|---|---|
| | (0.368) | (0.437) | (0.413) | (0.395) | (0.400) | (0.354) |
| Agreeableness$_H$ | 0.658 | 0.760 | 1.091$^{*}$ | 0.895 | 1.164$^{*}$ | 1.296$^{**}$ |
| | (0.501) | (0.537) | (0.535) | (0.507) | (0.566) | (0.475) |
| Agreeableness$_H$:Openness$_{AI}$ | -0.450 | -0.343 | -0.538 | -0.687 | -0.807 | -0.739$^{*}$ |
| | (0.380) | (0.421) | (0.411) | (0.397) | (0.427) | (0.374) |
| Agreeableness$_H$:Conscientiousness$_{AI}$ | -0.536 | -0.851$^{*}$ | -0.817$^{*}$ | -0.367 | -0.612 | -0.776$^{*}$ |
| | (0.376) | (0.416) | (0.415) | (0.415) | (0.430) | (0.375) |
| Agreeableness$_H$:Extraversion$_{AI}$ | 0.051 | 0.287 | 0.267 | -0.131 | 0.111 | 0.150 |
| | (0.362) | (0.392) | (0.391) | (0.369) | (0.398) | (0.345) |
| Agreeableness$_H$:Agreeableness$_{AI}$ | -0.301 | -0.417 | -0.096 | -0.158 | -0.192 | 0.042 |
| | (0.348) | (0.384) | (0.384) | (0.365) | (0.384) | (0.338) |
| Agreeableness$_H$:Neuroticism$_{AI}$ | 0.875$^{*}$ | 0.928$^{*}$ | 0.568 | 0.833$^{*}$ | 0.786$^{*}$ | 0.678 |
| | (0.347) | (0.392) | (0.384) | (0.374) | (0.393) | (0.349) |
| Neuroticism$_H$ | -0.424 | -0.440 | -0.876 | -0.209 | -0.074 | -0.305 |
| | (0.433) | (0.503) | (0.496) | (0.465) | (0.507) | (0.430) |
| Neuroticism$_H$:Openness$_{AI}$ | -0.086 | 0.404 | 0.485 | 0.307 | -0.016 | 0.038 |
| | (0.329) | (0.371) | (0.370) | (0.349) | (0.379) | (0.325) |
| Neuroticism$_H$:Conscientiousness$_{AI}$ | 0.161 | 0.043 | -0.028 | -0.154 | 0.060 | -0.289 |
| | (0.324) | (0.376) | (0.376) | (0.339) | (0.362) | (0.312) |
| Neuroticism$_H$:Extraversion$_{AI}$ | 0.276 | 0.090 | 0.357 | -0.198 | 0.214 | 0.259 |
| | (0.336) | (0.391) | (0.383) | (0.358) | (0.389) | (0.327) |
| Neuroticism$_H$:Agreeableness$_{AI}$ | 0.033 | 0.141 | 0.350 | 0.165 | 0.011 | 0.271 |
| | (0.322) | (0.360) | (0.356) | (0.338) | (0.343) | (0.306) |
| Neuroticism$_H$:Neuroticism$_{AI}$ | -0.256 | -0.641 | -0.551 | -0.273 | -0.527 | -0.424 |
| | (0.320) | (0.377) | (0.371) | (0.362) | (0.364) | (0.311) |
| Observations | 1,012 | 1,012 | 1,012 | 1,012 | 1,012 | 1,012 |

Notes: $^{*}p < 0.05$, $^{**}p < 0.01$, $^{***}p < 0.001$. Standard errors are heteroskedasticity robust. In the human-AI condition, 1,012 of the participants completed the post-task survey.

**Table S9. Regression table for Figure 3, the effects of human-AI personality interaction terms on ad quality measures.**

| | *text* | *image* | *click* |
|---|---|---|---|
| Intercept | 4.666$^{***}$ | 4.175$^{***}$ | 3.237$^{***}$ |
| | (0.226) | (0.212) | (0.215) |
| Openness$_{AI}$ | -0.009 | -0.054 | 0.102 |
| | (0.175) | (0.162) | (0.161) |
| Conscientiousness$_{AI}$ | -0.276 | 0.234 | 0.144 |
| | (0.169) | (0.161) | (0.157) |
| Extraversion$_{AI}$ | 0.310 | 0.171 | 0.102 |
| | (0.171) | (0.163) | (0.161) |
| Agreeableness$_{AI}$ | 0.599$^{***}$ | 0.149 | 0.141 |
| | (0.166) | (0.152) | (0.151) |
| Neuroticism$_{AI}$ | -0.133 | 0.021 | -0.035 |
| | (0.170) | (0.159) | (0.156) |
| Openness$_H$:Openness$_{AI}$ | 0.132 | -0.178 | -0.061 |
| | (0.117) | (0.116) | (0.112) |
| Openness$_H$:Conscientiousness$_{AI}$ | 0.262$^{*}$ | 0.110 | 0.144 |
| | (0.113) | (0.115) | (0.111) |
| Openness$_H$:Extraversion$_{AI}$ | -0.051 | -0.102 | -0.097 |
| | (0.113) | (0.116) | (0.112) |
| Openness$_H$:Agreeableness$_{AI}$ | -0.342$^{**}$ | 0.237$^{*}$ | 0.128 |

*Continued on next page*

*Table S9 (continued)*

| | *text* | *image* | *click* |
|---|---|---|---|
| | (0.113) | (0.111) | (0.108) |
| Openness$_H$ | 0.099 | 0.025 | -0.023 |
| | (0.139) | (0.141) | (0.138) |
| Openness$_H$:Neuroticism$_{AI}$ | 0.047 | 0.057 | 0.087 |
| | (0.114) | (0.113) | (0.110) |
| Conscientiousness$_H$ | 0.087 | -0.079 | 0.050 |
| | (0.191) | (0.189) | (0.187) |
| Conscientiousness$_H$:Openness$_{AI}$ | -0.145 | 0.369$^{*}$ | 0.042 |
| | (0.141) | (0.142) | (0.138) |
| Conscientiousness$_H$:Conscientiousness$_{AI}$ | 0.366$^{**}$ | 0.035 | 0.084 |
| | (0.138) | (0.141) | (0.136) |
| Conscientiousness$_H$:Extraversion$_{AI}$ | -0.157 | -0.011 | 0.014 |
| | (0.148) | (0.147) | (0.142) |
| Conscientiousness$_H$:Agreeableness$_{AI}$ | -0.483$^{**}$ | -0.274 | -0.299$^{*}$ |
| | (0.142) | (0.141) | (0.136) |
| Conscientiousness$_H$:Neuroticism$_{AI}$ | 0.165 | 0.059 | 0.122 |
| | (0.142) | (0.140) | (0.135) |
| Extraversion$_H$ | -0.079 | 0.113 | -0.052 |
| | (0.143) | (0.145) | (0.142) |
| Extraversion$_H$:Openness$_{AI}$ | 0.096 | 0.213 | 0.226 |
| | (0.123) | (0.121) | (0.118) |
| Extraversion$_H$:Conscientiousness$_{AI}$ | -0.437$^{***}$ | -0.447$^{***}$ | -0.397$^{**}$ |
| | (0.121) | (0.120) | (0.117) |
| Extraversion$_H$:Extraversion$_{AI}$ | 0.278$^{*}$ | -0.094 | 0.116 |
| | (0.119) | (0.120) | (0.117) |
| Extraversion$_H$:Agreeableness$_{AI}$ | 0.094 | -0.083 | 0.019 |
| | (0.122) | (0.119) | (0.118) |
| Extraversion$_H$:Neuroticism$_{AI}$ | -0.218 | 0.085 | -0.003 |
| | (0.122) | (0.120) | (0.118) |
| Agreeableness$_H$ | 0.091 | 0.269 | 0.274 |
| | (0.158) | (0.155) | (0.155) |
| Agreeableness$_H$:Openness$_{AI}$ | 0.032 | -0.287$^{*}$ | -0.157 |
| | (0.120) | (0.113) | (0.111) |
| Agreeableness$_H$:Conscientiousness$_{AI}$ | 0.075 | -0.065 | -0.020 |
| | (0.120) | (0.111) | (0.111) |
| Agreeableness$_H$:Extraversion$_{AI}$ | -0.387$^{**}$ | -0.091 | -0.216 |
| | (0.122) | (0.114) | (0.114) |
| Agreeableness$_H$:Agreeableness$_{AI}$ | -0.061 | 0.034 | 0.065 |
| | (0.122) | (0.112) | (0.113) |
| Agreeableness$_H$:Neuroticism$_{AI}$ | 0.262$^{*}$ | -0.106 | -0.095 |
| | (0.124) | (0.113) | (0.114) |
| Neuroticism$_H$ | 0.231 | 0.324$^{*}$ | 0.283$^{*}$ |
| | (0.143) | (0.145) | (0.142) |
| Neuroticism$_H$:Openness$_{AI}$ | -0.039 | 0.038 | -0.110 |
| | (0.117) | (0.110) | (0.105) |
| Neuroticism$_H$:Extraversion$_{AI}$ | 0.100 | 0.030 | 0.143 |
| | (0.114) | (0.109) | (0.105) |
| Neuroticism$_H$:Conscientiousness$_{AI}$ | -0.219 | -0.196 | -0.249$^{*}$ |
| | (0.113) | (0.107) | (0.101) |
| Neuroticism$_H$:Agreeableness$_{AI}$ | 0.003 | -0.179 | -0.071 |
| | (0.114) | (0.108) | (0.103) |
| Neuroticism$_H$:Neuroticism$_{AI}$ | -0.140 | -0.142 | -0.047 |
| | (0.117) | (0.109) | (0.103) |

*Continued on next page*

*Table S9 (continued)*

| | *text* | *image* | *click* |
|---|---|---|---|
| Observations | 30,126 | 30,126 | 30,126 |

Notes: $^{*}p < 0.05$, $^{**}p < 0.01$, $^{***}p < 0.001$. Standard errors are clustered on the ad level.

**Country of birth interactions** We further examine heterogeneity by country of birth by interacting AI personality prompts with region-of-birth indicators (*i.e.*, Western regions, East Asia, Latin America, Middle East & South Asia, etc.). The unit of observation is the rating, and we cluster standard errors at the ad level. Coefficients are interpretable as differential personality effects for each region relative to the omitted category. Full results are reported in Table S10.

**Table S10. Regression table for Figure 4, the effects of the interaction terms of a participants' country of birth and AI personality on ad quality measures.**

| | *text* | *image* | *click* |
|---|---|---|---|
| Intercept | 4.666$^{***}$ | 4.175$^{***}$ | 3.237$^{***}$ |
| | (0.226) | (0.212) | (0.215) |
| Openness$_{AI}$ | -0.009 | -0.054 | 0.102 |
| | (0.175) | (0.162) | (0.161) |
| Conscientiousness$_{AI}$ | -0.276 | 0.234 | 0.144 |
| | (0.169) | (0.161) | (0.157) |
| Extraversion$_{AI}$ | 0.310 | 0.171 | 0.102 |
| | (0.171) | (0.163) | (0.161) |
| Agreeableness$_{AI}$ | 0.599$^{***}$ | 0.149 | 0.141 |
| | (0.166) | (0.152) | (0.151) |
| Neuroticism$_{AI}$ | -0.133 | 0.021 | -0.035 |
| | (0.170) | (0.159) | (0.156) |
| Openness$_{H}$ | 0.099 | 0.025 | -0.023 |
| | (0.139) | (0.141) | (0.138) |
| Openness$_{H}$:Openness$_{AI}$ | 0.132 | -0.178 | -0.061 |
| | (0.117) | (0.116) | (0.112) |
| Openness$_{H}$:Conscientiousness$_{AI}$ | 0.262$^{*}$ | 0.110 | 0.144 |
| | (0.113) | (0.115) | (0.111) |
| Openness$_{H}$:Extraversion$_{AI}$ | -0.051 | -0.102 | -0.097 |
| | (0.113) | (0.116) | (0.112) |
| Openness$_{H}$:Agreeableness$_{AI}$ | -0.342$^{**}$ | 0.237$^{*}$ | 0.128 |
| | (0.113) | (0.111) | (0.108) |
| Openness$_{H}$:Neuroticism$_{AI}$ | 0.047 | 0.057 | 0.087 |
| | (0.114) | (0.113) | (0.110) |
| Conscientiousness$_{H}$ | 0.087 | -0.079 | 0.050 |
| | (0.191) | (0.189) | (0.187) |
| Conscientiousness$_{H}$:Openness$_{AI}$ | -0.145 | 0.369$^{*}$ | 0.042 |
| | (0.141) | (0.142) | (0.138) |
| Conscientiousness$_{H}$:Conscientiousness$_{AI}$ | 0.366$^{**}$ | 0.035 | 0.084 |
| | (0.138) | (0.141) | (0.136) |
| Conscientiousness$_{H}$:Extraversion$_{AI}$ | -0.157 | -0.011 | 0.014 |
| | (0.148) | (0.147) | (0.142) |
| Conscientiousness$_{H}$:Agreeableness$_{AI}$ | -0.483$^{**}$ | -0.274 | -0.299$^{*}$ |
| | (0.142) | (0.141) | (0.136) |
| Conscientiousness$_{H}$:Neuroticism$_{AI}$ | 0.165 | 0.059 | 0.122 |
| | (0.142) | (0.140) | (0.135) |
| Extraversion$_{H}$ | -0.079 | 0.113 | -0.052 |
| | (0.143) | (0.145) | (0.142) |
| Extraversion$_{H}$:Openness$_{AI}$ | 0.096 | 0.213 | 0.226 |
| | (0.123) | (0.121) | (0.118) |
| Extraversion$_{H}$:Conscientiousness$_{AI}$ | -0.437$^{***}$ | -0.447$^{***}$ | -0.397$^{**}$ |

*Continued on next page*

*Table S10 (continued)*

| | *text* | *image* | *click* |
|---|---|---|---|
| | (0.121) | (0.120) | (0.117) |
| Extraversion$_H$:Extraversion$_{AI}$ | 0.278$^*$ | -0.094 | 0.116 |
| | (0.119) | (0.120) | (0.117) |
| Extraversion$_H$:Agreeableness$_{AI}$ | 0.094 | -0.083 | 0.019 |
| | (0.122) | (0.119) | (0.118) |
| Extraversion$_H$:Neuroticism$_{AI}$ | -0.218 | 0.085 | -0.003 |
| | (0.122) | (0.120) | (0.118) |
| Agreeableness$_H$ | 0.091 | 0.269 | 0.274 |
| | (0.158) | (0.155) | (0.155) |
| Agreeableness$_H$:Openness$_{AI}$ | 0.032 | -0.287$^*$ | -0.157 |
| | (0.120) | (0.113) | (0.111) |
| Agreeableness$_H$:Conscientiousness$_{AI}$ | 0.075 | -0.065 | -0.020 |
| | (0.120) | (0.111) | (0.111) |
| Agreeableness$_H$:Extraversion$_{AI}$ | -0.387$^{**}$ | -0.091 | -0.216 |
| | (0.122) | (0.114) | (0.114) |
| Agreeableness$_H$:Agreeableness$_{AI}$ | -0.061 | 0.034 | 0.065 |
| | (0.122) | (0.112) | (0.113) |
| Agreeableness$_H$:Neuroticism$_{AI}$ | 0.262$^*$ | -0.106 | -0.095 |
| | (0.124) | (0.113) | (0.114) |
| Neuroticism$_H$ | 0.231 | 0.324$^*$ | 0.283$^*$ |
| | (0.143) | (0.145) | (0.142) |
| Neuroticism$_H$:Openness$_{AI}$ | -0.039 | 0.038 | -0.110 |
| | (0.117) | (0.110) | (0.105) |
| Neuroticism$_H$:Conscientiousness$_{AI}$ | -0.219 | -0.196 | -0.249$^*$ |
| | (0.113) | (0.107) | (0.101) |
| Neuroticism$_H$:Extraversion$_{AI}$ | 0.100 | 0.030 | 0.143 |
| | (0.114) | (0.109) | (0.105) |
| Neuroticism$_H$:Agreeableness$_{AI}$ | 0.003 | -0.179 | -0.071 |
| | (0.114) | (0.108) | (0.103) |
| Neuroticism$_H$:Neuroticism$_{AI}$ | -0.140 | -0.142 | -0.047 |
| | (0.117) | (0.109) | (0.103) |
| Observations | 30,126 | 30,126 | 30,126 |

Notes: $^*p < 0.05$, $^{**}p < 0.01$, $^{***}p < 0.001$. Standard errors are clustered on the ad level.

**Productivity** We model individual productivity as the number of ads submitted within the 40-minute session. Specifications include human traits and demographics, with heteroskedasticity-robust standard errors at the individual level. Interaction terms between human and AI personality quantify how pairings shape output volume. Full results are reported in Table S11.

**Table S11. Regression table for Figure 5, the effects of human-AI personality interaction terms on productivity.**

| | *number of submissions* |
|---|---|
| Intercept | 8.400$^*$ |
| | (3.317) |
| Openness$_{AI}$ | -0.834 |
| | (2.372) |
| Conscientiousness$_{AI}$ | -0.734 |
| | (2.316) |
| Extraversion$_{AI}$ | 0.593 |
| | (2.268) |
| Agreeableness$_{AI}$ | -3.606 |
| | (2.405) |
| Neuroticism$_{AI}$ | 2.596 |
| | (2.367) |

*Continued on next page*

*Table S11 (continued)*

| | *number of submissions* |
|---|---|
| $\text{Openness}_H$ | 1.754 |
| | (1.627) |
| $\text{Openness}_H$:$\text{Openness}_{AI}$ | -1.314 |
| | (1.371) |
| $\text{Openness}_H$:$\text{Conscientiousness}_{AI}$ | 0.004 |
| | (1.326) |
| $\text{Openness}_H$:$\text{Extraversion}_{AI}$ | -0.187 |
| | (1.316) |
| $\text{Openness}_H$:$\text{Agreeableness}_{AI}$ | -0.839 |
| | (1.369) |
| $\text{Openness}_H$:$\text{Neuroticism}_{AI}$ | -0.021 |
| | (1.329) |
| $\text{Conscientiousness}_H$ | -0.265 |
| | (2.909) |
| $\text{Conscientiousness}_H$:$\text{Openness}_{AI}$ | -0.391 |
| | (2.265) |
| $\text{Conscientiousness}_H$:$\text{Conscientiousness}_{AI}$ | -1.566 |
| | (2.395) |
| $\text{Conscientiousness}_H$:$\text{Extraversion}_{AI}$ | -1.359 |
| | (2.254) |
| $\text{Conscientiousness}_H$:$\text{Agreeableness}_{AI}$ | 1.251 |
| | (2.264) |
| $\text{Conscientiousness}_H$:$\text{Neuroticism}_{AI}$ | -0.617 |
| | (2.400) |
| $\text{Extraversion}_H$ | -2.345 |
| | (1.789) |
| $\text{Extraversion}_H$:$\text{Openness}_{AI}$ | -0.969 |
| | (1.401) |
| $\text{Extraversion}_H$:$\text{Conscientiousness}_{AI}$ | 1.868 |
| | (1.389) |
| $\text{Extraversion}_H$:$\text{Extraversion}_{AI}$ | -0.371 |
| | (1.352) |
| $\text{Extraversion}_H$:$\text{Agreeableness}_{AI}$ | 2.986$^{*}$ |
| | (1.388) |
| $\text{Extraversion}_H$:$\text{Neuroticism}_{AI}$ | 1.349 |
| | (1.353) |
| $\text{Agreeableness}_H$ | -0.730 |
| | (2.258) |
| $\text{Agreeableness}_H$:$\text{Openness}_{AI}$ | 3.543$^{*}$ |
| | (1.717) |
| $\text{Agreeableness}_H$:$\text{Conscientiousness}_{AI}$ | 0.783 |
| | (1.410) |
| $\text{Agreeableness}_H$:$\text{Extraversion}_{AI}$ | 0.088 |
| | (1.442) |
| $\text{Agreeableness}_H$:$\text{Agreeableness}_{AI}$ | 0.062 |
| | (1.410) |
| $\text{Agreeableness}_H$:$\text{Neuroticism}_{AI}$ | -3.725$^{*}$ |
| | (1.719) |
| $\text{Neuroticism}_H$ | -3.620$^{*}$ |
| | (1.823) |
| $\text{Neuroticism}_H$:$\text{Openness}_{AI}$ | 0.975 |
| | (1.228) |
| $\text{Neuroticism}_H$:$\text{Conscientiousness}_{AI}$ | 0.842 |
| | (1.289) |
| $\text{Neuroticism}_H$:$\text{Extraversion}_{AI}$ | 1.067 |

*Continued on next page*

*Table S11 (continued)*

| | *number of submissions* |
|---|---|
| | (1.181) |
| Neuroticism$_H$:Agreeableness$_{AI}$ | 2.950$^*$ |
| | (1.157) |
| Neuroticism$_H$:Neuroticism$_{AI}$ | -0.127 |
| | (1.323) |
| Observations | 1,222 |

Notes: $^*p < 0.05$, $^{**}p < 0.01$, $^{***}p < 0.001$. Standard errors are heteroskedasticity robust. In the human-AI condition, 1,222 of the participants submitted ads.

**I. Regression tables for AI use and employment status.** To study heterogeneity by prior AI exposure, we interacted AI personality prompts with *Used AI* and *Positive AI Experience* indicators and estimated rating-level regressions with ad-level clustered standard errors (Table S12). To study heterogeneity by employment status, we interacted AI personality prompts with Prolific employment categories and estimated the same specification (Table S13). Across moderators, point estimates and standard errors quantify how personality effects vary with user background.

**Table S12. Regression table for Figure S5, the effects of the interaction terms of a participants' previous AI experience and AI personality on ad quality measures.**

| | *text* | *image* | *click* |
|---|---|---|---|
| Intercept | $4.893^{***}$ | $4.522^{***}$ | $3.492^{***}$ |
| | (0.092) | (0.101) | (0.096) |
| $\text{Openness}_{AI}$ | 0.089 | -0.069 | 0.054 |
| | (0.084) | (0.082) | (0.080) |
| $\text{Conscientiousness}_{AI}$ | $-0.249^{**}$ | -0.055 | -0.070 |
| | (0.084) | (0.081) | (0.079) |
| $\text{Extraversion}_{AI}$ | $0.271^{**}$ | 0.123 | $0.181^{*}$ |
| | (0.085) | (0.085) | (0.081) |
| $\text{Agreeableness}_{AI}$ | 0.008 | 0.008 | 0.004 |
| | (0.090) | (0.085) | (0.082) |
| $\text{Neuroticism}_{AI}$ | $-0.261^{**}$ | $-0.223^{**}$ | $-0.224^{**}$ |
| | (0.084) | (0.081) | (0.080) |
| Used AI | $0.514^{**}$ | 0.021 | 0.263 |
| | (0.197) | (0.219) | (0.206) |
| Used AI $\times$ $\text{Openness}_{AI}$ | $-0.486^{**}$ | 0.091 | -0.065 |
| | (0.185) | (0.192) | (0.186) |
| Used AI $\times$ $\text{Conscientiousness}_{AI}$ | $0.418^{*}$ | 0.041 | 0.053 |
| | (0.186) | (0.187) | (0.180) |
| Used AI $\times$ $\text{Extraversion}_{AI}$ | $-0.577^{**}$ | $-0.376^{*}$ | $-0.443^{*}$ |
| | (0.173) | (0.180) | (0.175) |
| Used AI $\times$ $\text{Agreeableness}_{AI}$ | $-0.470^{**}$ | 0.148 | -0.066 |
| | (0.177) | (0.184) | (0.177) |
| Used AI $\times$ $\text{Neuroticism}_{AI}$ | $0.708^{***}$ | $0.503^{**}$ | $0.514^{**}$ |
| | (0.173) | (0.181) | (0.179) |
| Used AI $\times$ Positive AI Experience | $-0.080^{**}$ | -0.005 | -0.033 |
| | (0.029) | (0.032) | (0.030) |
| Used AI $\times$ Positive AI Experience $\times$ $\text{Openness}_{AI}$ | $0.080^{**}$ | 0.005 | 0.015 |
| | (0.027) | (0.028) | (0.028) |
| Used AI $\times$ Positive AI Experience $\times$ $\text{Conscientiousness}_{AI}$ | -0.043 | -0.001 | -0.001 |
| | (0.027) | (0.028) | (0.027) |
| Used AI $\times$ Positive AI Experience $\times$ $\text{Extraversion}_{AI}$ | $0.058^{*}$ | 0.040 | 0.043 |
| | (0.025) | (0.026) | (0.026) |
| Used AI $\times$ Positive AI Experience $\times$ $\text{Agreeableness}_{AI}$ | $0.080^{**}$ | -0.025 | 0.014 |
| | (0.026) | (0.027) | (0.026) |
| Used AI $\times$ Positive AI Experience $\times$ $\text{Neuroticism}_{AI}$ | $-0.069^{**}$ | -0.041 | -0.041 |
| | (0.025) | (0.027) | (0.026) |
| Observations | 27,129 | 27,129 | 27,129 |

Notes: $^{*}p < 0.05$, $^{**}p < 0.01$, $^{***}p < 0.001$. Standard errors are clustered on the ad level. Ads and their ratings were included only for individuals who submitted the post-task survey.

**Table S13. Regression table for Figure S6, the effects of the interaction terms of a participants' employment status and AI personality on ad quality measures.**

| | *text* | *image* | *click* |
|---|---|---|---|
| Intercept | $4.987^{***}$ | $4.543^{***}$ | $3.645^{***}$ |

*Continued on next page*

*Table S13 (continued)*

| | *text* | *image* | *click* |
|---|---|---|---|
| | (0.112) | (0.112) | (0.113) |
| $\text{Openness}_{AI}$ | -0.174* | 0.090 | -0.020 |
| | (0.081) | (0.085) | (0.087) |
| $\text{Conscientiousness}_{AI}$ | -0.184* | -0.006 | -0.042 |
| | (0.080) | (0.082) | (0.080) |
| $\text{Extraversion}_{AI}$ | 0.327*** | 0.105 | 0.165 |
| | (0.079) | (0.087) | (0.085) |
| $\text{Agreeableness}_{AI}$ | -0.102 | -0.134 | -0.049 |
| | (0.082) | (0.084) | (0.087) |
| $\text{Neuroticism}_{AI}$ | 0.094 | -0.039 | -0.047 |
| | (0.087) | (0.082) | (0.083) |
| Full-time × $\text{Openness}_{AI}$ | 0.263** | 0.033 | 0.155 |
| | (0.089) | (0.092) | (0.093) |
| Full-time × $\text{Conscientiousness}_{AI}$ | 0.061 | -0.023 | 0.020 |
| | (0.089) | (0.090) | (0.087) |
| Full-time × $\text{Extraversion}_{AI}$ | -0.251** | -0.066 | -0.115 |
| | (0.087) | (0.094) | (0.092) |
| Full-time × $\text{Agreeableness}_{AI}$ | 0.161 | 0.141 | 0.070 |
| | (0.090) | (0.091) | (0.094) |
| Full-time × $\text{Neuroticism}_{AI}$ | -0.104 | 0.086 | 0.108 |
| | (0.095) | (0.089) | (0.090) |
| Full-time | -0.154 | -0.129 | -0.227 |
| | (0.121) | (0.121) | (0.121) |
| Part-time × $\text{Openness}_{AI}$ | 0.361** | -0.108 | 0.087 |
| | (0.106) | (0.113) | (0.112) |
| Part-time × $\text{Conscientiousness}_{AI}$ | 0.196 | -0.027 | -0.008 |
| | (0.105) | (0.111) | (0.107) |
| Part-time × $\text{Extraversion}_{AI}$ | -0.402*** | -0.211 | -0.192 |
| | (0.104) | (0.114) | (0.111) |
| Part-time × $\text{Agreeableness}_{AI}$ | 0.009 | -0.047 | -0.071 |
| | (0.106) | (0.112) | (0.113) |
| Part-time × $\text{Neuroticism}_{AI}$ | -0.179 | 0.050 | 0.037 |
| | (0.110) | (0.110) | (0.109) |
| Part-time | 0.088 | 0.187 | 0.076 |
| | (0.138) | (0.142) | (0.144) |
| Other × $\text{Openness}_{AI}$ | -0.132 | -0.417** | -0.218 |
| | (0.137) | (0.151) | (0.150) |
| Other × $\text{Conscientiousness}_{AI}$ | 0.574*** | -0.008 | 0.272 |
| | (0.139) | (0.160) | (0.150) |
| Other × $\text{Extraversion}_{AI}$ | -0.173 | 0.008 | 0.016 |
| | (0.140) | (0.160) | (0.154) |
| Other × $\text{Agreeableness}_{AI}$ | 0.064 | 0.278 | 0.087 |
| | (0.144) | (0.151) | (0.153) |
| Other × $\text{Neuroticism}_{AI}$ | 0.030 | 0.192 | 0.211 |
| | (0.146) | (0.165) | (0.155) |
| Other | -0.117 | -0.028 | -0.204 |
| | (0.175) | (0.177) | (0.174) |
| Starting soon × $\text{Openness}_{AI}$ | -0.975*** | -0.845 | -0.950* |
| | (0.262) | (0.480) | (0.471) |
| Starting soon × $\text{Conscientiousness}_{AI}$ | -0.506* | -0.111 | -0.230 |
| | (0.232) | (0.359) | (0.391) |
| Starting soon × $\text{Extraversion}_{AI}$ | -1.475** | -0.022 | -0.039 |
| | (0.447) | (0.427) | (0.491) |
| Starting soon × $\text{Agreeableness}_{AI}$ | 0.384 | 0.926* | 1.089** |
| | (0.269) | (0.398) | (0.327) |

*Continued on next page*

*Table S13 (continued)*

| | *text* | *image* | *click* |
|---|---|---|---|
| Starting soon × Neuroticism$_{AI}$ | 1.979$^{***}$ | 0.906 | 0.973 |
| | (0.397) | (0.566) | (0.569) |
| Starting soon | 0.921$^{*}$ | -0.017 | 0.146 |
| | (0.394) | (0.431) | (0.480) |
| Seeking work | 0.047 | 0.306 | 0.187 |
| | (0.159) | (0.157) | (0.156) |
| Seeking work × Openness$_{AI}$ | 0.198 | -0.115 | 0.079 |
| | (0.108) | (0.116) | (0.116) |
| Seeking work × Conscientiousness$_{AI}$ | 0.070 | -0.030 | -0.013 |
| | (0.111) | (0.116) | (0.113) |
| Seeking work × Extraversion$_{AI}$ | -0.283$^{**}$ | -0.306$^{*}$ | -0.304$^{**}$ |
| | (0.108) | (0.119) | (0.116) |
| Seeking work × Agreeableness$_{AI}$ | 0.119 | 0.082 | 0.043 |
| | (0.109) | (0.118) | (0.116) |
| Seeking work × Neuroticism$_{AI}$ | -0.114 | -0.260$^{*}$ | -0.148 |
| | (0.115) | (0.116) | (0.114) |
| Observations | 26,291 | 26,291 | 26,291 |

Notes: $^{*}p < 0.05$, $^{**}p < 0.01$, $^{***}p < 0.001$. Standard errors are clustered on the ad level. Ads and their ratings were included only for individuals whose employment status was not "Unknown" on Prolific.

**J. Average treatment effects.** We report average treatment effects (ATEs) of the AI personality prompts on (i) ad quality (human ratings of text, image, click; Table S14), (ii) productivity (submissions; Table S15), and (iii) teamwork quality dimensions (Table S16). For ad ratings, standard errors are clustered at the ad level; for productivity and teamwork, we use heteroskedasticity-robust standard errors at the individual level.

**Table S14. Average treatment effects of personality prompts on performance.**

| | *text* | *image* | *click* |
|---|---|---|---|
| Intercept | 4.917*** | 4.495*** | 3.533*** |
| | (0.031) | (0.032) | (0.031) |
| $\text{Openness}_{AI}$ | 0.038 | 0.030 | 0.059* |
| | (0.025) | (0.025) | (0.024) |
| $\text{Conscientiousness}_{AI}$ | -0.094*** | -0.002 | -0.011 |
| | (0.025) | (0.025) | (0.024) |
| $\text{Extraversion}_{AI}$ | 0.089*** | 0.018 | 0.032 |
| | (0.025) | (0.025) | (0.024) |
| $\text{Agreeableness}_{AI}$ | 0.018 | 0.008 | 0.020 |
| | (0.025) | (0.025) | (0.024) |
| $\text{Neuroticism}_{AI}$ | 0.000 | 0.004 | 0.014 |
| | (0.025) | (0.025) | (0.024) |
| Observations | 30126 | 30126 | 30126 |

Notes: *p<0.05; **p<0.01; ***p<0.001. Standard errors are clustered on the ad level.

**Table S15. Average treatment effects of personality prompts on productivity.**

| | *Submission* |
|---|---|
| Intercept | 5.831*** |
| | (0.343) |
| $\text{Openness}_{AI}$ | 0.324 |
| | (0.300) |
| $\text{Conscientiousness}_{AI}$ | 0.001 |
| | (0.303) |
| $\text{Extraversion}_{AI}$ | -0.216 |
| | (0.297) |
| $\text{Agreeableness}_{AI}$ | -0.039 |
| | (0.298) |
| $\text{Neuroticism}_{AI}$ | 0.158 |
| | (0.300) |
| Observations | 1222 |

Notes: *p<0.05; **p<0.01; ***p<0.001. Heteroskedasticity-robust standard errors are reported.

**Table S16. Average treatment effects of personality prompts on teamwork.**

| | *communication* | *coordination* | *balance* | *mutual support* | *effort* | *cohesion* |
|---|---|---|---|---|---|---|
| Intercept | 5.627*** | 5.426*** | 5.370*** | 5.733*** | 5.756*** | 5.340*** |
| | (0.083) | (0.091) | (0.089) | (0.084) | (0.092) | (0.081) |
| Openness$_{AI}$ | -0.063 | -0.001 | 0.014 | -0.036 | -0.040 | -0.059 |
| | (0.065) | (0.071) | (0.072) | (0.066) | (0.072) | (0.065) |
| Conscientiousness$_{AI}$ | 0.025 | 0.026 | -0.005 | 0.021 | -0.040 | 0.015 |
| | (0.065) | (0.072) | (0.072) | (0.067) | (0.073) | (0.065) |
| Extraversion$_{AI}$ | 0.024 | 0.010 | -0.089 | -0.003 | 0.049 | 0.031 |
| | (0.065) | (0.072) | (0.072) | (0.067) | (0.073) | (0.065) |
| Agreeableness$_{AI}$ | -0.039 | -0.051 | 0.032 | 0.011 | -0.073 | 0.028 |
| | (0.065) | (0.072) | (0.072) | (0.067) | (0.073) | (0.065) |
| Neuroticism$_{AI}$ | 0.062 | 0.142* | 0.134 | 0.115 | 0.084 | 0.070 |
| | (0.065) | (0.071) | (0.072) | (0.067) | (0.073) | (0.065) |
| Observations | 1012 | 1012 | 1012 | 1012 | 1012 | 1012 |

Notes: $^{*}p<0.05$; $^{**}p<0.01$; $^{***}p<0.001$. Heteroskedasticity-robust standard errors are reported.

**K. Field results.** We evaluate downstream ad performance on X using mixed-effects models with campaign random effects to account for unobserved heterogeneity across 400 campaigns. For CPC, we exclude ads with zero clicks as CPC is undefined in those cases (as noted in the table footers). Explanatory variables include human-rated text, image, and click measures and spend to accommodate auto-bidding dynamics. Table S17 presents results for CPC and CTR, while Table S18 presents results for view-through rate (fraction of report viewed) and view-through duration (log-seconds) measured via DocSend links unique to each ad.

**Table S17. Regression table for the effects of the human-AI personality pairing on real-world click-through rates (CTR) and cost-per-click (CPC) from the field study.**

| | CTR (%) | | | CPC ($) | | |
|---|---|---|---|---|---|---|
| Intercept | -0.067 | -0.072*** | -0.141* | 14.211*** | 12.693*** | 16.533*** |
| | (0.057) | (0.018) | (0.059) | (2.920) | (0.938) | (3.041) |
| Image | | 0.006 | 0.005 | | -0.538** | -0.461** |
| | | (0.003) | (0.003) | | (0.175) | (0.178) |
| Text | | 0.011*** | 0.012*** | | -0.253 | -0.314 |
| | | (0.003) | (0.003) | | (0.165) | (0.169) |
| Click | | -0.006 | -0.006 | | 0.465* | 0.470* |
| | | (0.004) | (0.004) | | (0.196) | (0.198) |
| Openness$_{AI}$ | 0.062 | | 0.068 | 2.523 | | 2.290 |
| | (0.044) | | (0.044) | (2.268) | | (2.261) |
| Conscientiousness$_{AI}$ | -0.002 | | 0.004 | -2.175 | | -1.972 |
| | (0.046) | | (0.045) | (2.315) | | (2.313) |
| Extraversion$_{AI}$ | -0.007 | | -0.004 | -0.495 | | -0.583 |
| | (0.045) | | (0.045) | (2.313) | | (2.304) |
| Agreeableness$_{AI}$ | 0.027 | | 0.013 | -4.779* | | -4.457 |
| | (0.045) | | (0.045) | (2.311) | | (2.312) |
| Neuroticism$_{AI}$ | -0.017 | | -0.008 | -0.911 | | -1.431 |
| | (0.046) | | (0.045) | (2.327) | | (2.326) |
| Openness$_{H}$ | 0.048 | | 0.051 | -1.354 | | -1.425 |
| | (0.034) | | (0.033) | (1.722) | | (1.718) |
| Conscientiousness$_{H}$ | 0.088* | | 0.084 | -1.797 | | -1.913 |
| | (0.045) | | (0.045) | (2.300) | | (2.295) |
| Extraversion$_{H}$ | -0.023 | | -0.020 | -3.003 | | -2.936 |
| | (0.035) | | (0.035) | (1.849) | | (1.845) |
| Agreeableness$_{H}$ | -0.038 | | -0.034 | 1.108 | | 1.087 |
| | (0.041) | | (0.040) | (2.082) | | (2.077) |
| Neuroticism$_{H}$ | -0.002 | | -0.002 | -1.295 | | -1.381 |
| | (0.037) | | (0.037) | (1.906) | | (1.898) |
| Openness$_{AI}$:Openness$_{H}$ | -0.035 | | -0.044 | -0.287 | | -0.082 |
| | (0.028) | | (0.028) | (1.424) | | (1.428) |
| Openness$_{AI}$:Conscientiousness$_{H}$ | 0.001 | | -0.002 | -0.695 | | -0.405 |
| | (0.034) | | (0.034) | (1.737) | | (1.734) |
| Openness$_{AI}$:Extraversion$_{H}$ | 0.017 | | 0.025 | -2.166 | | -2.394 |
| | (0.029) | | (0.029) | (1.502) | | (1.498) |
| Openness$_{AI}$:Agreeableness$_{H}$ | -0.044 | | -0.046 | -0.781 | | -0.788 |
| | (0.031) | | (0.031) | (1.584) | | (1.578) |
| Openness$_{AI}$:Neuroticism$_{H}$ | -0.028 | | -0.025 | -0.545 | | -0.655 |
| | (0.028) | | (0.027) | (1.423) | | (1.418) |
| Conscientiousness$_{AI}$:Openness$_{H}$ | 0.025 | | 0.027 | 0.525 | | 0.494 |
| | (0.028) | | (0.028) | (1.426) | | (1.420) |
| Conscientiousness$_{AI}$:Conscientiousness$_{H}$ | -0.040 | | -0.041 | 1.083 | | 0.931 |
| | (0.034) | | (0.034) | (1.771) | | (1.766) |
| Conscientiousness$_{AI}$:Extraversion$_{H}$ | -0.004 | | -0.009 | 1.178 | | 1.116 |
| | (0.029) | | (0.029) | (1.502) | | (1.503) |
| Conscientiousness$_{AI}$:Agreeableness$_{H}$ | 0.021 | | 0.022 | 0.624 | | 0.512 |
| | (0.031) | | (0.031) | (1.572) | | (1.568) |

*Continued on next page*

*Table S17 (continued)*

| | | CTR (%) | | | CPC ($) | |
|---|---|---|---|---|---|---|
| Conscientiousness$_{AI}$:Neuroticism$_{H}$ | 0.011 | | 0.006 | -0.579 | | -0.568 |
| | (0.028) | | (0.028) | (1.450) | | (1.448) |
| Extraversion$_{AI}$:Openness$_{H}$ | -0.031 | | -0.033 | 2.151 | | 2.095 |
| | (0.028) | | (0.027) | (1.420) | | (1.416) |
| Extraversion$_{AI}$:Conscientiousness$_{H}$ | -0.036 | | -0.035 | 1.315 | | 1.477 |
| | (0.034) | | (0.034) | (1.747) | | (1.743) |
| Extraversion$_{AI}$:Extraversion$_{H}$ | 0.041 | | 0.042 | -0.836 | | -1.005 |
| | (0.029) | | (0.029) | (1.522) | | (1.517) |
| Extraversion$_{AI}$:Agreeableness$_{H}$ | 0.054 | | 0.050 | -2.511 | | -2.314 |
| | (0.032) | | (0.031) | (1.619) | | (1.614) |
| Extraversion$_{AI}$:Neuroticism$_{H}$ | -0.016 | | -0.017 | 1.466 | | 1.361 |
| | (0.029) | | (0.029) | (1.486) | | (1.482) |
| Agreeableness$_{AI}$:Openness$_{H}$ | -0.010 | | -0.005 | 0.688 | | 0.458 |
| | (0.027) | | (0.027) | (1.388) | | (1.385) |
| Agreeableness$_{AI}$:Conscientiousness$_{H}$ | -0.029 | | -0.024 | 0.247 | | 0.231 |
| | (0.033) | | (0.033) | (1.728) | | (1.725) |
| Agreeableness$_{AI}$:Extraversion$_{H}$ | -0.019 | | -0.020 | 2.991 | | 3.105* |
| | (0.030) | | (0.029) | (1.542) | | (1.537) |
| Agreeableness$_{AI}$:Agreeableness$_{H}$ | 0.003 | | 0.013 | 2.789 | | 2.415 |
| | (0.032) | | (0.032) | (1.625) | | (1.625) |
| Agreeableness$_{AI}$:Neuroticism$_{H}$ | 0.016 | | 0.021 | 1.530 | | 1.570 |
| | (0.029) | | (0.029) | (1.510) | | (1.510) |
| Neuroticism$_{AI}$:Openness$_{H}$ | -0.004 | | -0.008 | -1.907 | | -1.645 |
| | (0.028) | | (0.028) | (1.421) | | (1.420) |
| Neuroticism$_{AI}$:Conscientiousness$_{H}$ | -0.072* | | -0.068* | 3.531* | | 3.537* |
| | (0.034) | | (0.034) | (1.764) | | (1.758) |
| Neuroticism$_{AI}$:Extraversion$_{H}$ | 0.055 | | 0.056 | 0.588 | | 0.483 |
| | (0.029) | | (0.028) | (1.485) | | (1.480) |
| Neuroticism$_{AI}$:Agreeableness$_{H}$ | 0.031 | | 0.020 | -1.877 | | -1.479 |
| | (0.031) | | (0.031) | (1.590) | | (1.589) |
| Neuroticism$_{AI}$:Neuroticism$_{H}$ | 0.059* | | 0.056* | 0.956 | | 1.156 |
| | (0.028) | | (0.028) | (1.443) | | (1.439) |
| Spend | 0.007*** | 0.008*** | 0.008*** | -0.144*** | -0.151*** | -0.150*** |
| | (0.000) | (0.000) | (0.000) | (0.019) | (0.019) | (0.020) |
| Campaign RE | Yes | Yes | Yes | Yes | Yes | Yes |
| Observations | 1152 | 1152 | 1152 | 1068 | 1068 | 1068 |

Notes: $^{*}p < 0.05$, $^{**}p < 0.01$, $^{***}p < 0.001$. Campaign RE represents campaign random effects. Ads with zero clicks were removed for regressions for columns 3-4.

**Table S18. Regression table for the effects of the human-AI personality pairing on real-world view-through rates (VTR; fraction of report) and view-through duration (VTD; log-seconds) on DocSend.**

| | | VTR | | | VTD (log-sec) | |
|---|---|---|---|---|---|---|
| Intercept | 0.124$^{*}$ | 0.043$^{**}$ | 0.132$^{*}$ | 0.915 | 0.418$^{**}$ | 0.877 |
| | (0.051) | (0.013) | (0.053) | (0.538) | (0.137) | (0.566) |
| Image | | -0.001 | -0.003 | | 0.027 | 0.020 |
| | | (0.003) | (0.003) | | (0.033) | (0.035) |
| Text | | 0.001 | 0.002 | | 0.039 | 0.037 |
| | | (0.003) | (0.003) | | (0.028) | (0.030) |
| Click | | -0.003 | -0.002 | | -0.064 | -0.056 |
| | | (0.004) | (0.004) | | (0.037) | (0.039) |

*Continued on next page*

*Table S18 (continued)*

| | VTR | | VTD (log-sec) | |
|---|---|---|---|---|
| $\text{Openness}_{AI}$ | -0.064 | -0.063 | -0.403 | -0.348 |
| | (0.040) | (0.041) | (0.424) | (0.437) |
| $\text{Conscientiousness}_{AI}$ | -0.030 | -0.027 | 0.171 | 0.114 |
| | (0.041) | (0.041) | (0.431) | (0.446) |
| $\text{Extraversion}_{AI}$ | -0.000 | -0.002 | -0.072 | -0.064 |
| | (0.041) | (0.041) | (0.434) | (0.448) |
| $\text{Agreeableness}_{AI}$ | -0.035 | -0.033 | -0.444 | -0.493 |
| | (0.043) | (0.043) | (0.447) | (0.459) |
| $\text{Neuroticism}_{AI}$ | -0.011 | -0.016 | -0.148 | -0.142 |
| | (0.040) | (0.041) | (0.428) | (0.447) |
| $\text{Openness}_{H}$ | 0.060 | $0.062^{*}$ | 0.125 | 0.124 |
| | (0.031) | (0.031) | (0.321) | (0.330) |
| $\text{Conscientiousness}_{H}$ | -0.058 | -0.059 | 0.080 | 0.108 |
| | (0.040) | (0.040) | (0.417) | (0.428) |
| $\text{Extraversion}_{H}$ | $-0.086^{**}$ | $-0.085^{**}$ | -0.326 | -0.338 |
| | (0.033) | (0.033) | (0.342) | (0.351) |
| $\text{Agreeableness}_{H}$ | -0.008 | -0.005 | -0.296 | -0.315 |
| | (0.037) | (0.037) | (0.390) | (0.401) |
| $\text{Neuroticism}_{H}$ | -0.047 | -0.049 | -0.156 | -0.239 |
| | (0.034) | (0.034) | (0.356) | (0.367) |
| $\text{Openness}_{AI}$:$\text{Openness}_{H}$ | -0.019 | -0.021 | -0.349 | -0.388 |
| | (0.025) | (0.026) | (0.265) | (0.274) |
| $\text{Openness}_{AI}$:$\text{Conscientiousness}_{H}$ | $0.064^{*}$ | $0.066^{*}$ | 0.526 | 0.467 |
| | (0.031) | (0.031) | (0.325) | (0.335) |
| $\text{Openness}_{AI}$:$\text{Extraversion}_{H}$ | 0.030 | 0.029 | 0.009 | -0.017 |
| | (0.027) | (0.027) | (0.282) | (0.290) |
| $\text{Openness}_{AI}$:$\text{Agreeableness}_{H}$ | -0.018 | -0.018 | 0.004 | 0.034 |
| | (0.028) | (0.028) | (0.293) | (0.302) |
| $\text{Openness}_{AI}$:$\text{Neuroticism}_{H}$ | 0.034 | 0.035 | 0.360 | 0.389 |
| | (0.025) | (0.025) | (0.259) | (0.268) |
| $\text{Conscientiousness}_{AI}$:$\text{Openness}_{H}$ | $-0.051^{*}$ | $-0.053^{*}$ | -0.491 | -0.500 |
| | (0.025) | (0.025) | (0.265) | (0.273) |
| $\text{Conscientiousness}_{AI}$:$\text{Conscientiousness}_{H}$ | 0.014 | 0.014 | 0.140 | 0.170 |
| | (0.031) | (0.031) | (0.320) | (0.332) |
| $\text{Conscientiousness}_{AI}$:$\text{Extraversion}_{H}$ | 0.036 | 0.034 | -0.053 | -0.037 |
| | (0.027) | (0.027) | (0.279) | (0.287) |
| $\text{Conscientiousness}_{AI}$:$\text{Agreeableness}_{H}$ | 0.029 | 0.027 | 0.145 | 0.160 |
| | (0.028) | (0.028) | (0.293) | (0.302) |
| $\text{Conscientiousness}_{AI}$:$\text{Neuroticism}_{H}$ | 0.016 | 0.016 | -0.139 | -0.099 |
| | (0.025) | (0.025) | (0.261) | (0.269) |
| $\text{Extraversion}_{AI}$:$\text{Openness}_{H}$ | -0.006 | -0.007 | 0.362 | 0.362 |
| | (0.025) | (0.026) | (0.266) | (0.273) |
| $\text{Extraversion}_{AI}$:$\text{Conscientiousness}_{H}$ | 0.028 | 0.031 | -0.146 | -0.188 |
| | (0.031) | (0.031) | (0.321) | (0.331) |
| $\text{Extraversion}_{AI}$:$\text{Extraversion}_{H}$ | -0.001 | -0.002 | 0.074 | 0.130 |
| | (0.028) | (0.028) | (0.288) | (0.296) |
| $\text{Extraversion}_{AI}$:$\text{Agreeableness}_{H}$ | -0.008 | -0.008 | -0.039 | -0.056 |
| | (0.029) | (0.029) | (0.303) | (0.313) |
| $\text{Extraversion}_{AI}$:$\text{Neuroticism}_{H}$ | -0.023 | -0.022 | -0.195 | -0.175 |
| | (0.026) | (0.026) | (0.276) | (0.285) |
| $\text{Agreeableness}_{AI}$:$\text{Openness}_{H}$ | -0.018 | -0.018 | 0.192 | 0.176 |
| | (0.025) | (0.025) | (0.258) | (0.264) |
| $\text{Agreeableness}_{AI}$:$\text{Conscientiousness}_{H}$ | 0.009 | 0.009 | 0.091 | 0.092 |
| | (0.030) | (0.030) | (0.316) | (0.326) |

*Continued on next page*

*Table S18 (continued)*

| | VTR | | | VTD (log-sec) | | |
|---|---|---|---|---|---|---|
| Agreeableness$_{AI}$:Extraversion$_{H}$ | 0.018 | | 0.019 | 0.007 | | 0.018 |
| | (0.027) | | (0.027) | (0.288) | | (0.297) |
| Agreeableness$_{AI}$:Agreeableness$_{H}$ | 0.026 | | 0.023 | 0.209 | | 0.264 |
| | (0.030) | | (0.030) | (0.314) | | (0.323) |
| Agreeableness$_{AI}$:Neuroticism$_{H}$ | 0.013 | | 0.012 | 0.026 | | 0.074 |
| | (0.027) | | (0.027) | (0.286) | | (0.294) |
| Neuroticism$_{AI}$:Openness$_{H}$ | 0.004 | | 0.007 | -0.074 | | -0.040 |
| | (0.025) | | (0.026) | (0.267) | | (0.275) |
| Neuroticism$_{AI}$:Conscientiousness$_{H}$ | -0.022 | | -0.021 | -0.156 | | -0.153 |
| | (0.031) | | (0.031) | (0.325) | | (0.334) |
| Neuroticism$_{AI}$:Extraversion$_{H}$ | 0.040 | | 0.042 | 0.254 | | 0.282 |
| | (0.027) | | (0.027) | (0.279) | | (0.287) |
| Neuroticism$_{AI}$:Agreeableness$_{H}$ | -0.001 | | -0.001 | 0.155 | | 0.104 |
| | (0.028) | | (0.028) | (0.298) | | (0.307) |
| Neuroticism$_{AI}$:Neuroticism$_{H}$ | 0.007 | | 0.009 | 0.195 | | 0.180 |
| | (0.025) | | (0.025) | (0.261) | | (0.271) |
| Spend | 0.000 | 0.000 | 0.000 | 0.003 | 0.003$^{*}$ | 0.002 |
| | (0.000) | (0.000) | (0.000) | (0.002) | (0.001) | (0.002) |
| Campaign RE | Yes | Yes | Yes | Yes | Yes | Yes |
| Observations | 2760 | 2760 | 2760 | 2760 | 2760 | 2760 |

Notes: $^{*}p < 0.05$, $^{**}p < 0.01$, $^{***}p < 0.001$. Campaign RE represents campaign random effects. Observations are document views.

## References


1. S Noy, W Zhang, Experimental evidence on the productivity effects of generative artificial intelligence. *Science* **381**, 187–192 (2023).
2. E Wiles, ZT Munyikwa, JJ Horton, Algorithmic writing assistance on jobseekers' resumes increases hires, (National Bureau of Economic Research), Working Paper 30886 (2023).
3. E Brynjolfsson, D Li, LR Raymond, Generative ai at work, (National Bureau of Economic Research), Working Paper 31161 (2023).
4. F Dell'Acqua, et al., Navigating the jagged technological frontier: Field experimental evidence of the effects of ai on knowledge worker productivity and quality, (Harvard Business School), Working Paper 24-013 (2023).
5. H Ju, S Aral, Collaborating with ai agents: Field experiments on teamwork, productivity, and performance (2025).
6. M Chen, et al., Impact of human and artificial intelligence collaboration on workload reduction in medical image interpretation. *NPJ Digit. Medicine* **7**, 349 (2024).
7. F Yu, et al., Heterogeneity and predictors of the effects of ai assistance on radiologists. *Nat. Medicine* **30**, 837–849 (2024).
8. S Krakowski, D Haftor, J Luger, N Pashkevich, S Raisch, Human-centered artificial intelligence: A field experiment. *Manag. Sci.* **0** (2025).
9. MR Barrick, GL Stewart, MJ Neubert, MK Mount, Relating member ability and personality to work-team processes and team effectiveness. *J. applied psychology* **83**, 377 (1998).
10. ST Bell, Deep-level composition variables as predictors of team performance: a meta-analysis. *J. applied psychology* **92**, 595 (2007).
11. SL Kichuk, WH Wiesner, The big five personality factors and team performance: implications for selecting successful product design teams. *J. Eng. Technol. management* **14**, 195–221 (1997).
12. MA Peeters, CG Rutte, HF van Tuijl, IM Reymen, The big five personality traits and individual satisfaction with the team. *Small group research* **37**, 187–211 (2006).
13. AW Woolley, CF Chabris, A Pentland, N Hashmi, TW Malone, Evidence for a collective intelligence factor in the performance of human groups. *Science* **330**, 686–688 (2010).
14. AW Woolley, RM Chow, AT Mayo, C Riedl, JW Chang, Collective attention and collective intelligence: The role of hierarchy and team gender composition. *Organ. Sci.* **34**, 1315–1331 (2023).
15. EE Makarius, D Mukherjee, JD Fox, AK Fox, Rising with the machines: A sociotechnical framework for bringing artificial intelligence into the organization. *Organ. & Mark. Policies & Process. eJournal* **120** (2020).
16. G Zhang, L Chong, K Kotovsky, J Cagan, Trust in an ai versus a human teammate: The effects of teammate identity and performance on human-ai cooperation. *Comput. Hum. Behav.* **139**, 107536 (2023).
17. A Fügener, J Grahl, A Gupta, W Ketter, Cognitive challenges in human–artificial intelligence collaboration: Investigating the path toward productive delegation. *Inf. Syst. Res.* **33**, 678–696 (2022).
18. P Hemmer, et al., Human-ai collaboration: The effect of ai delegation on human task performance and task satisfaction in *Proceedings of the 28th International Conference on Intelligent User Interfaces*, IUI '23. (ACM), (2023).
19. C Anthony, BA Bechky, AL Fayard, "collaborating" with ai: Taking a system view to explore the future of work. *Organ. Sci.* **34**, 1672–1694 (2023).
20. KM Collins, et al., Building machines that learn and think with people. *Nat. Hum. Behav.* **8**, 1851–1863 (2024).
21. B Li, EY Lai, X Wang, Express: From tools to agents: Meta-analytic insights into human acceptance of ai. *J. Mark.* **0**, 00222429251355266 (2025).
22. MF Jung, et al., Engaging robots: easing complex human-robot teamwork using backchanneling in *Proceedings of the 2013 Conference on Computer Supported Cooperative Work*, CSCW '13. (Association for Computing Machinery, New York, NY, USA), p. 1555–1566 (2013).
23. M Jung, P Hinds, Robots in the wild: A time for more robust theories of human-robot interaction. *J. Hum.-Robot Interact.* **7** (2018).
24. CM Fang, et al., How ai and human behaviors shape psychosocial effects of chatbot use: A longitudinal randomized controlled study (2025).
25. OpenAI, Sycophancy in GPT-4o (https://openai.com/index/sycophancy-in-gpt-4o/) (2025) Accessed: 2025-08-29.
26. OpenAI, Customizing your ChatGPT personality (https://help.openai.com/en/articles/11899719-customizing-your-chatgpt-personality) (2025) Accessed: 2025-08-29.
27. Anthropic, Claude character (https://www.anthropic.com/research/claude-character) (2024) Accessed: 2025-08-29.
28. M Sharma, et al., Towards understanding sycophancy in language models (2025).
29. K Gelbrich, H Roschk, S Miederer, A Kerath, Express: Automated versus human agents: A meta-analysis of customer responses to robots, chatbots, and algorithms and their contingencies. *J. Mark.* **0**, 00222429251344139 (2025).
30. W Wang, G Gao, R Agarwal, Friend or foe? teaming between artificial intelligence and workers with variation in experience. *Manag. Sci.* **70**, 5753–5775 (2023).
31. A Humlum, E Vestergaard, The adoption of chatgpt, (University of Chicago, Becker Friedman Institute for Economics), Working Paper 2024-50 (2024).
32. N Otis, R Clarke, S Delecourt, D Holtz, R Koning, The uneven impact of generative ai on entrepreneurial performance (2024) Available at SSRN: https://ssrn.com/abstract=4671369.
33. N Agarwal, A Moehring, P Rajpurkar, T Salz, Combining human expertise with artificial intelligence: Experimental

evidence from radiology, (National Bureau of Economic Research), Technical report (2023).
34. M Vaccaro, A Almaatouq, T Malone, When combinations of humans and ai are useful: A systematic review and meta-analysis. *Nat. Hum. Behav.* **8** (2024).
35. A Sergeyuk, I Zakharov, E Koshchenko, M Izadi, Human-ai experience in integrated development environments: A systematic literature review (2025).
36. TB Brown, et al., Language models are few-shot learners (2020).
37. J Wei, et al., Chain-of-thought prompting elicits reasoning in large language models in *Advances in Neural Information Processing Systems*, eds. S Koyejo, et al. (Curran Associates, Inc.), Vol. 35, pp. 24824–24837 (2022).
38. R Chen, A Arditi, H Sleight, O Evans, J Lindsey, Persona vectors: Monitoring and controlling character traits in language models (2025).
39. S Schulhoff, et al., The prompt report: A systematic survey of prompting techniques (2024).
40. G Jiang, et al., Evaluating and inducing personality in pre-trained language models (2023).
41. B Rammstedt, OP John, Measuring personality in one minute or less: A 10-item short version of the big five inventory in english and german. *J. Res. Pers.* **41**, 203–212 (2007).
42. M Hoegl, HG Gemuenden, Teamwork quality and the success of innovative projects: A theoretical concept and empirical evidence. *Organ. Sci.* **12**, 435–449 (2001).
